# Supplementary material for: Conditions for Suppression of Gas Phase Chemical Reactions inside a Dark Infrared Cavity: O$_{2}$ + 2NO$\to$ 2NO$_{2}$ as an example
Source: arXiv:2509.03299 source file (2025-09-03)
Supplement: Supplementary file 1 [file SI.tex]

\begin{center}
    \Large\textbf{Conditions for Suppression of Gas Phase Chemical Reactions inside a Dark Infrared Cavity: O$_{2}$ + 2NO → 2NO$_{2}$ as an Example}

    Mwdansar Banuary, Ashish Kumar Gupta, Nimrod Moiseyev$\text{*}$

\Huge{\textbf{Supplementary Information}}
\end{center}

\newpage

The reaction that has been studied is
\begin{equation}
    2NO + O_{2} \rightarrow 2NO_{2}
\end{equation}

The mechanism of the above reaction followed in the calculation is

Step 1
\begin{equation}
    NO+O_{2} \rightarrow NO_{3} 
\end{equation}

Step 2
\begin{equation}
    NO_{3} + NO \rightarrow 2NO_{2} 
\end{equation}

The calculation of potential energy surface is carried out using Gaussian 16 at B3LYP/6-31G(d) level. In step 1, we get two transition states (TS1 and TS2). IRC curves for TS1 and TS2 are shown in Figs. \ref{SIfig_1} and \ref{SIfig_2} respectively. Both IRCs go up to optimized points except towards the reactant. Some points are added from the relax scan of the distance between the center of mass of NO molecule and the center of mass of O$_{2}$ molecule following the Generalized Internal Coordinates (GIC) approach to the IRC of TS1 towards the reactant to connect to the optimized structure of the reactant (Fig. \ref{SIfig_3}). Connecting the IRCs and the points obtained from the relax scan, a complete potential energy curve for the step 1 reaction is obtained (Fig. \ref{SIfig_31}).

\begin{figure}[H]
\centering
  \includegraphics[width=\linewidth]{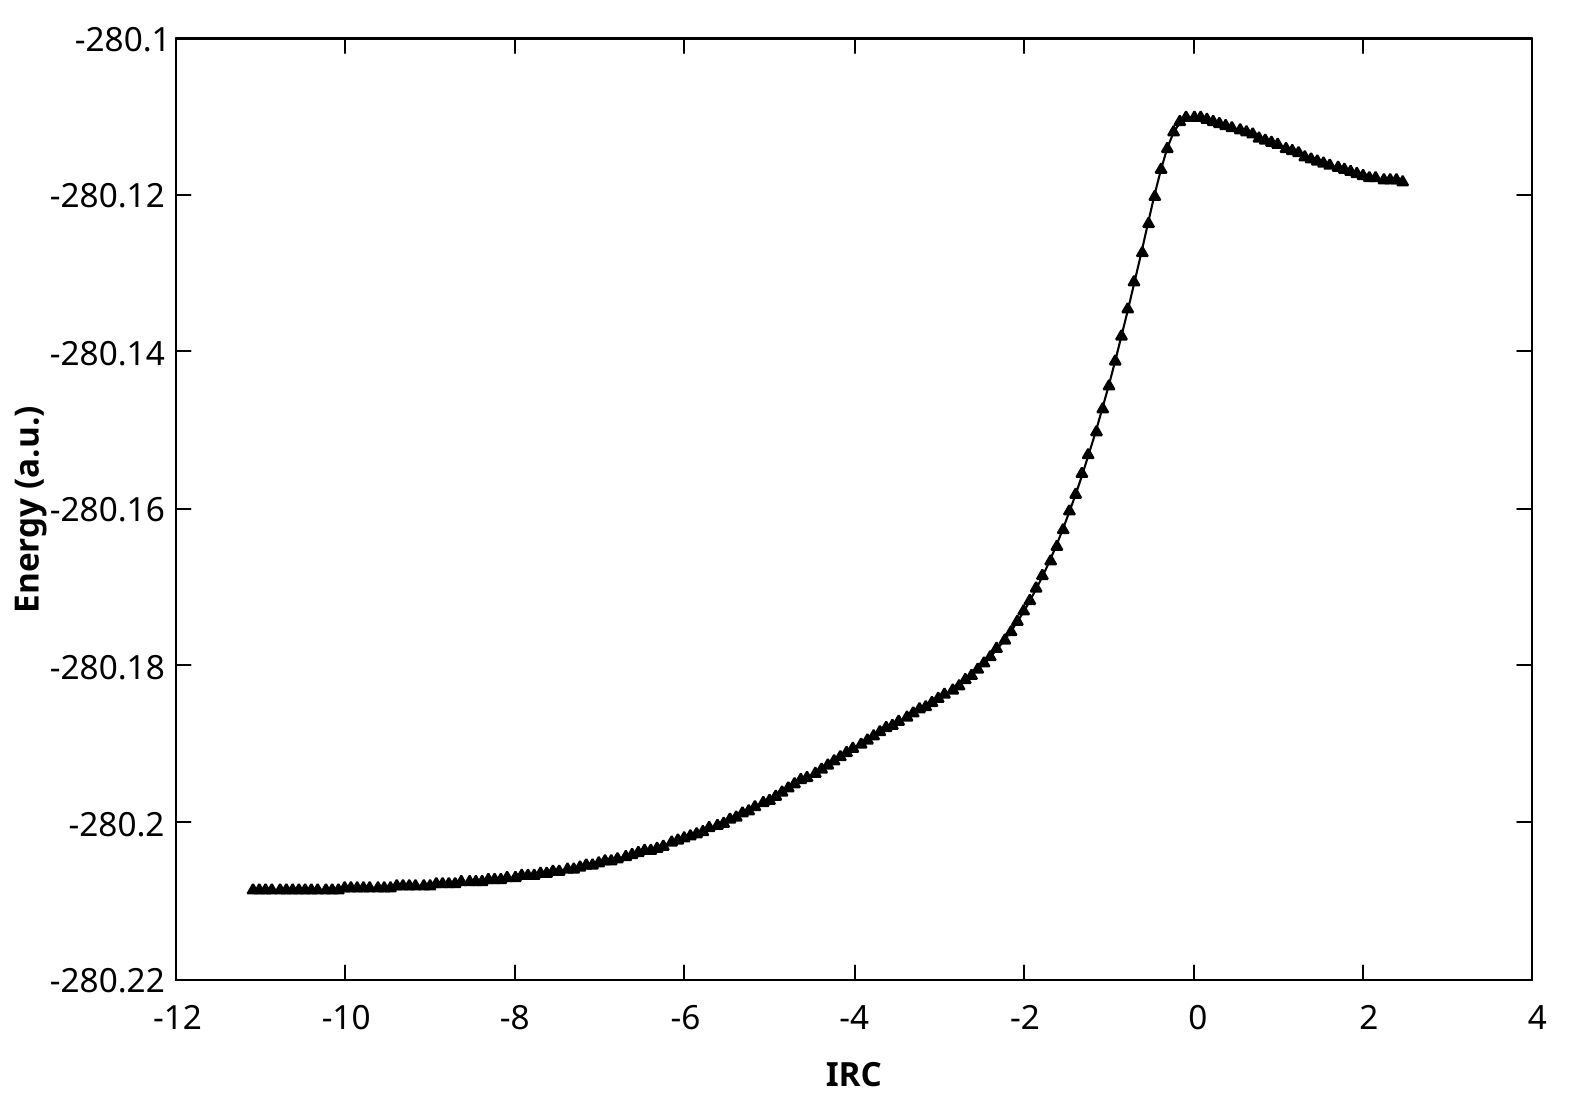}
  \caption{IRC curve of TS1 for step 1 reaction which is showing (from left to right): O$_{2}$+NO $\rightarrow$ TS1 $\rightarrow$ INT.}
  \label{SIfig_1}
\end{figure}

\begin{figure}[H]
\centering
  \includegraphics[width=\linewidth]{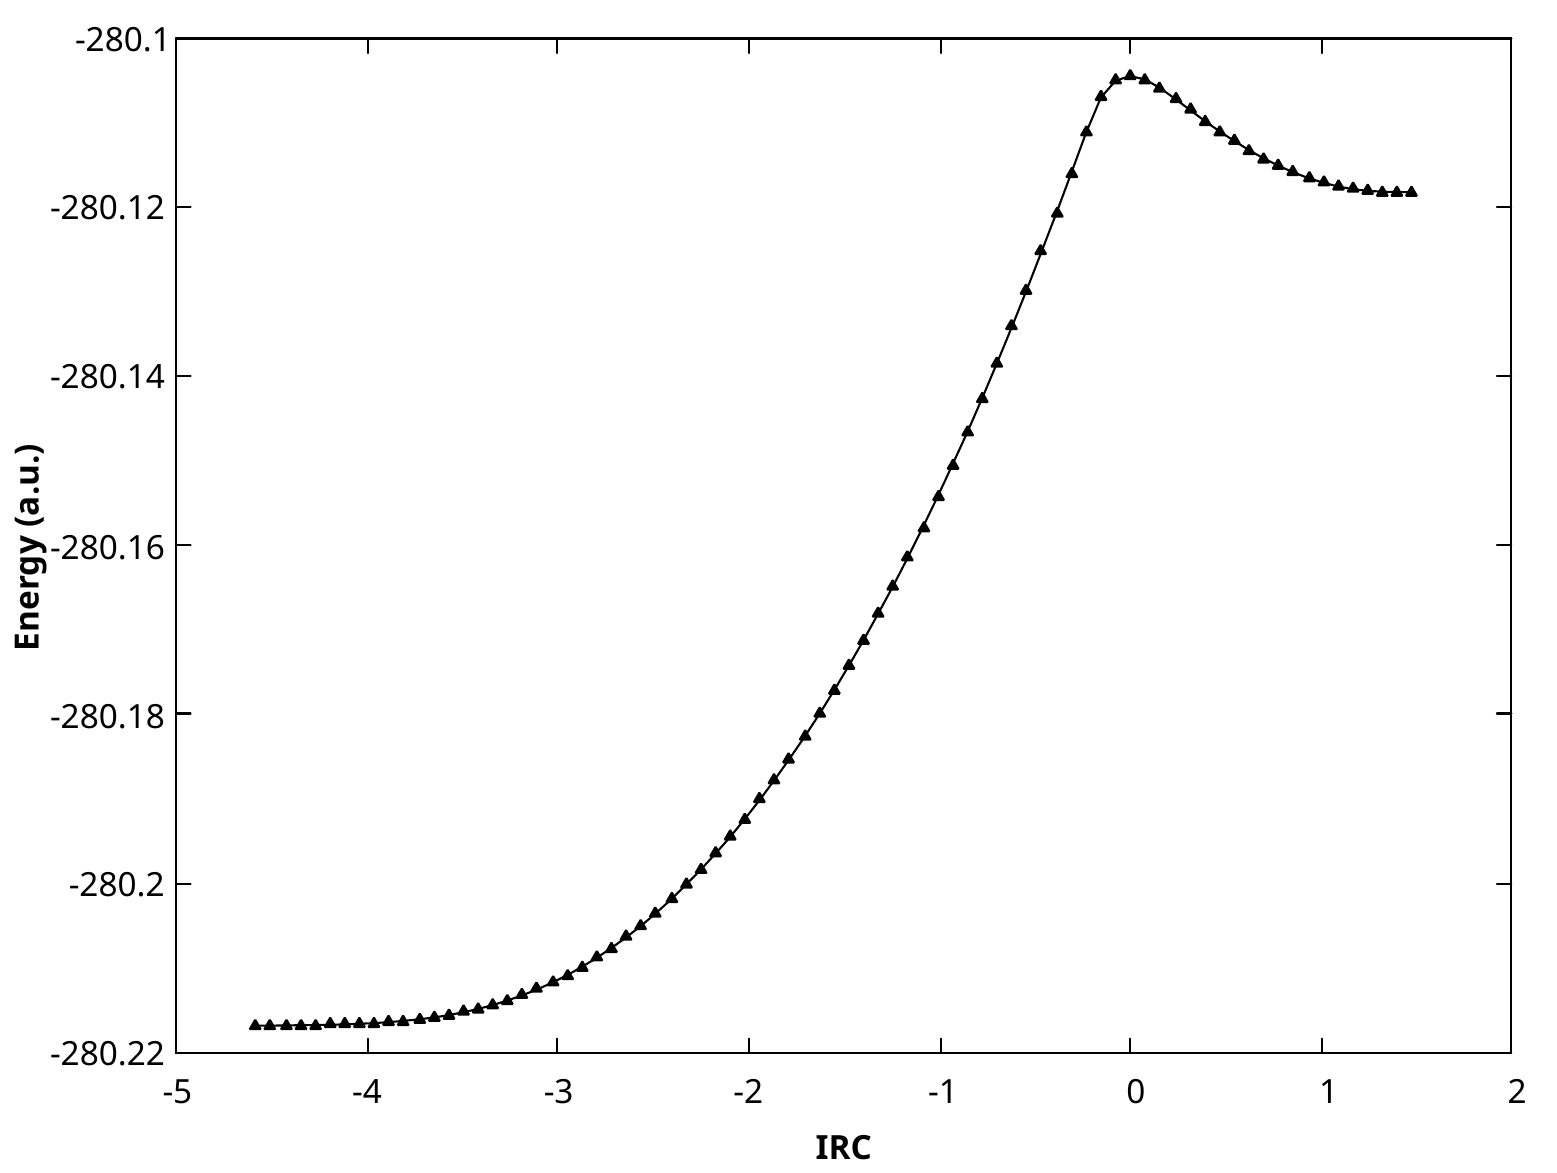}
  \caption{IRC curve of TS2 for step 1 reaction which is showing (from left to right): NO$_{3}$ $\rightarrow$ TS2 $\rightarrow$ INT (INT is same as shown in Fig. \ref{SIfig_1}.)}
  \label{SIfig_2}
\end{figure}

\begin{figure}[H]
\centering
  \includegraphics[width=\linewidth]{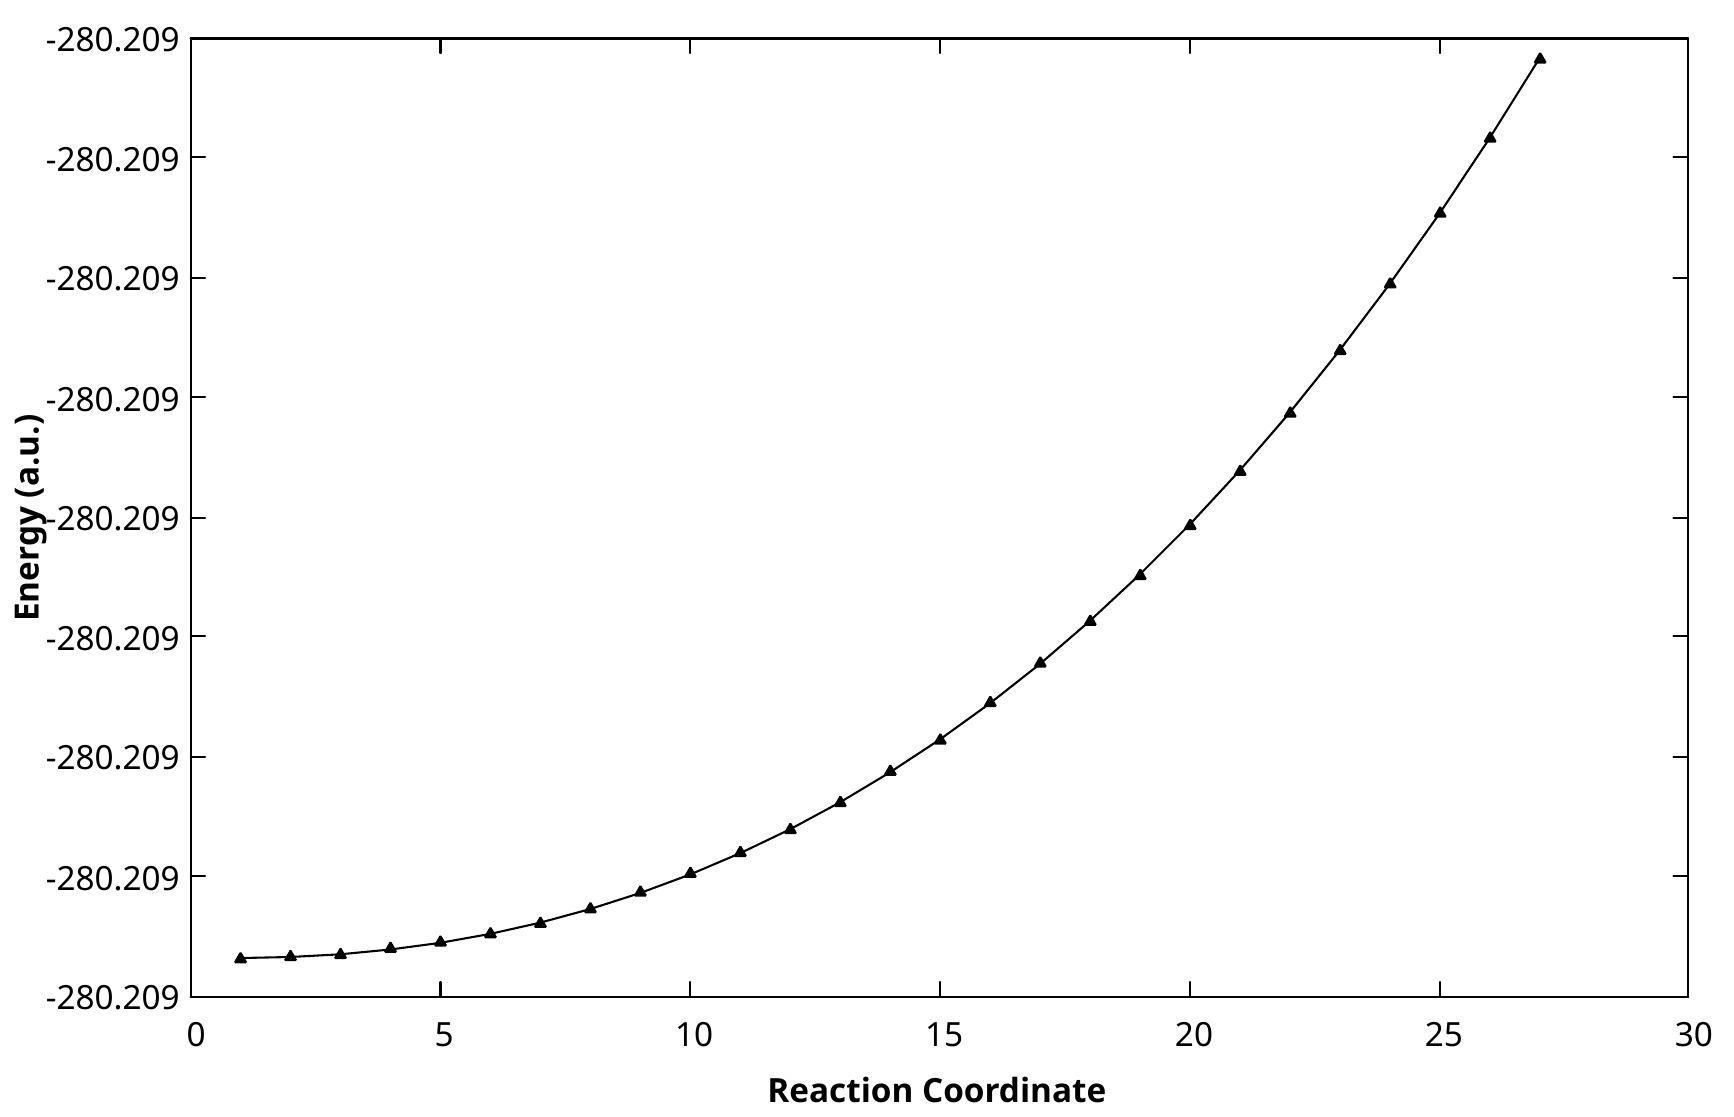}
  \caption{Relax scan of distance between the center of mass of NO and O$_{2}$ molecules to connect last point of IRC of TS1 towards reactant to optimized reactant.}
  \label{SIfig_3}
\end{figure}

\begin{figure}[H]
\centering
  \includegraphics[width=\linewidth]{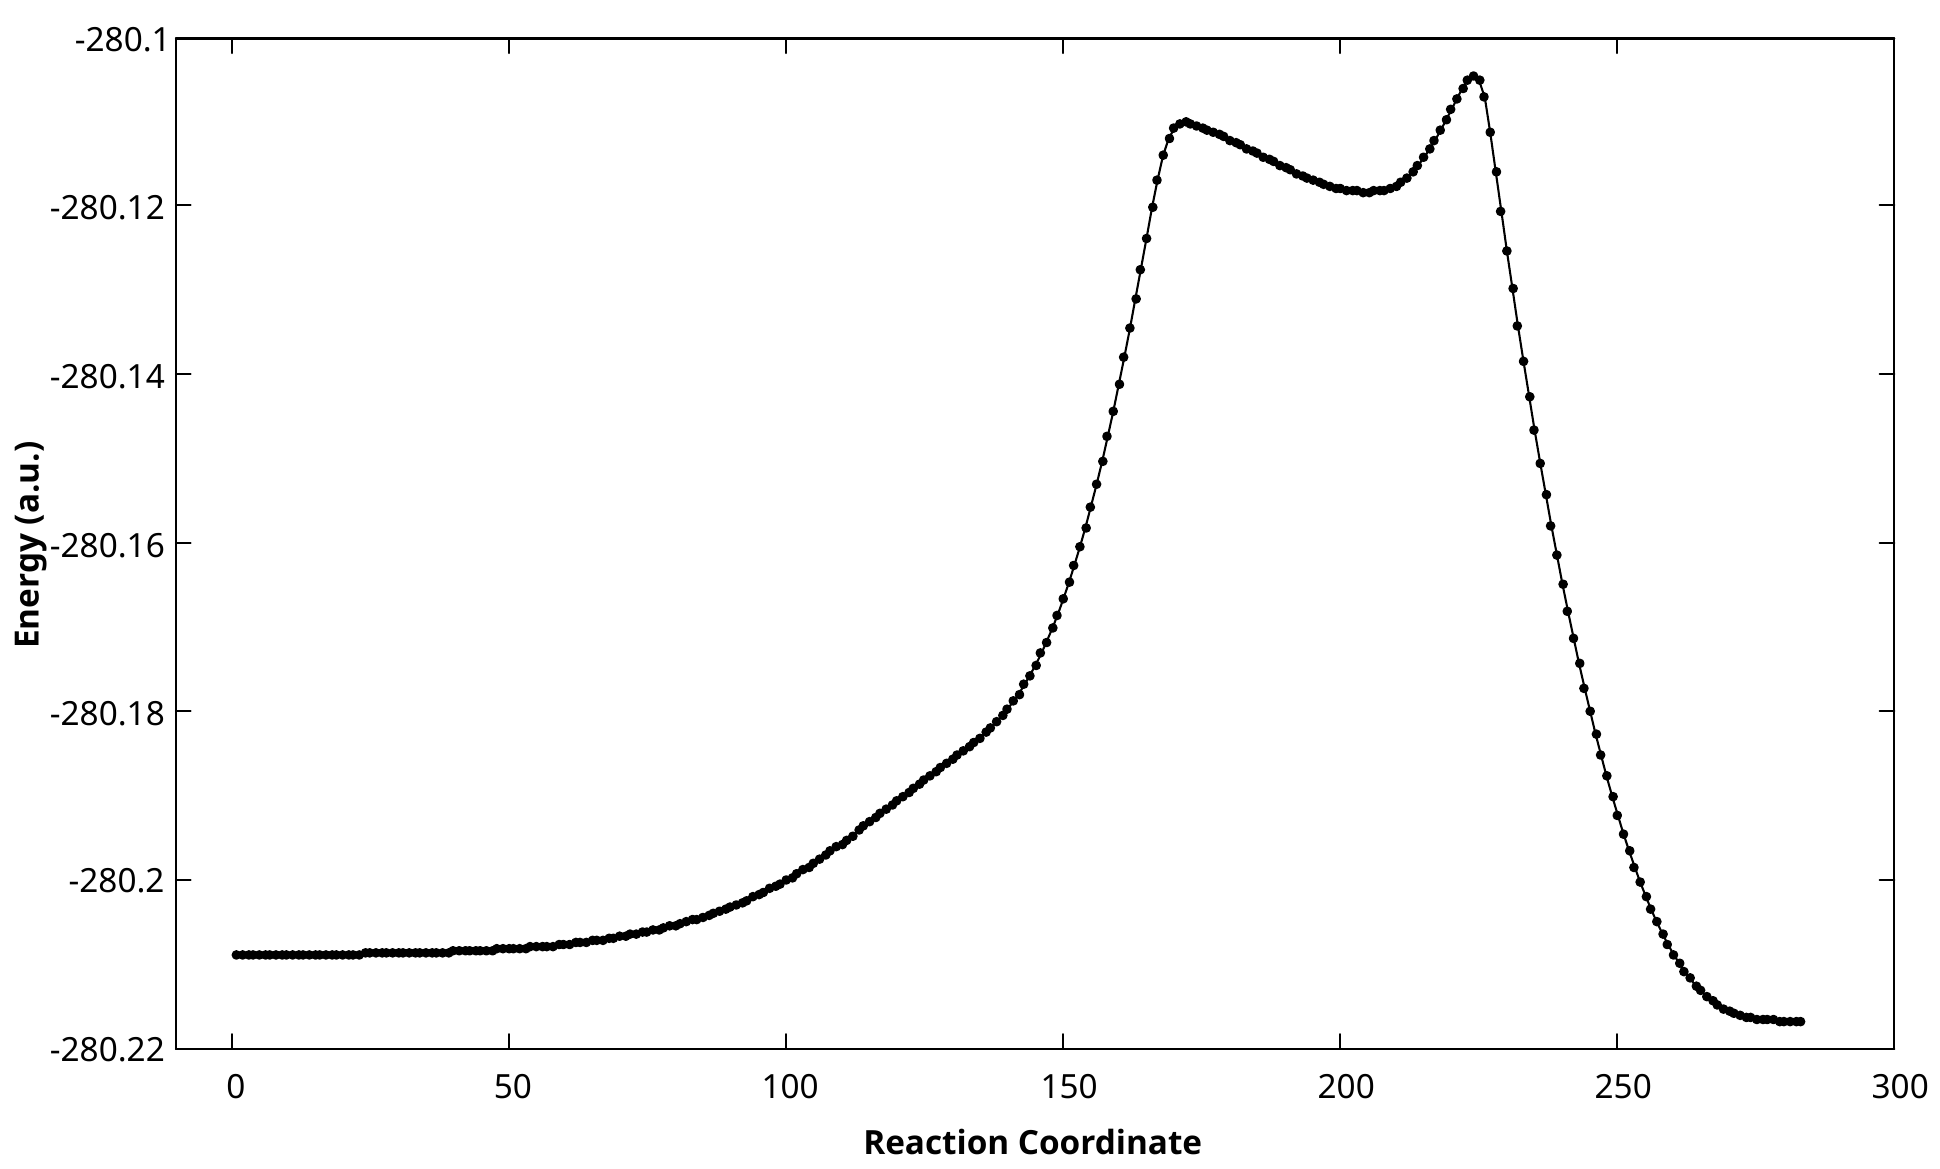}
  \caption{Potential energy curve for step 1 reaction which is showing (from left to right): O$_{2}$+NO $\rightarrow$ TS1 $\rightarrow$ INT $\rightarrow$ TS2 $\rightarrow$ NO$_{3}$.}
  \label{SIfig_31}
\end{figure}

\begin{figure}[H]
  \centering
  \subfigure[]{\includegraphics[width=0.3\textwidth]{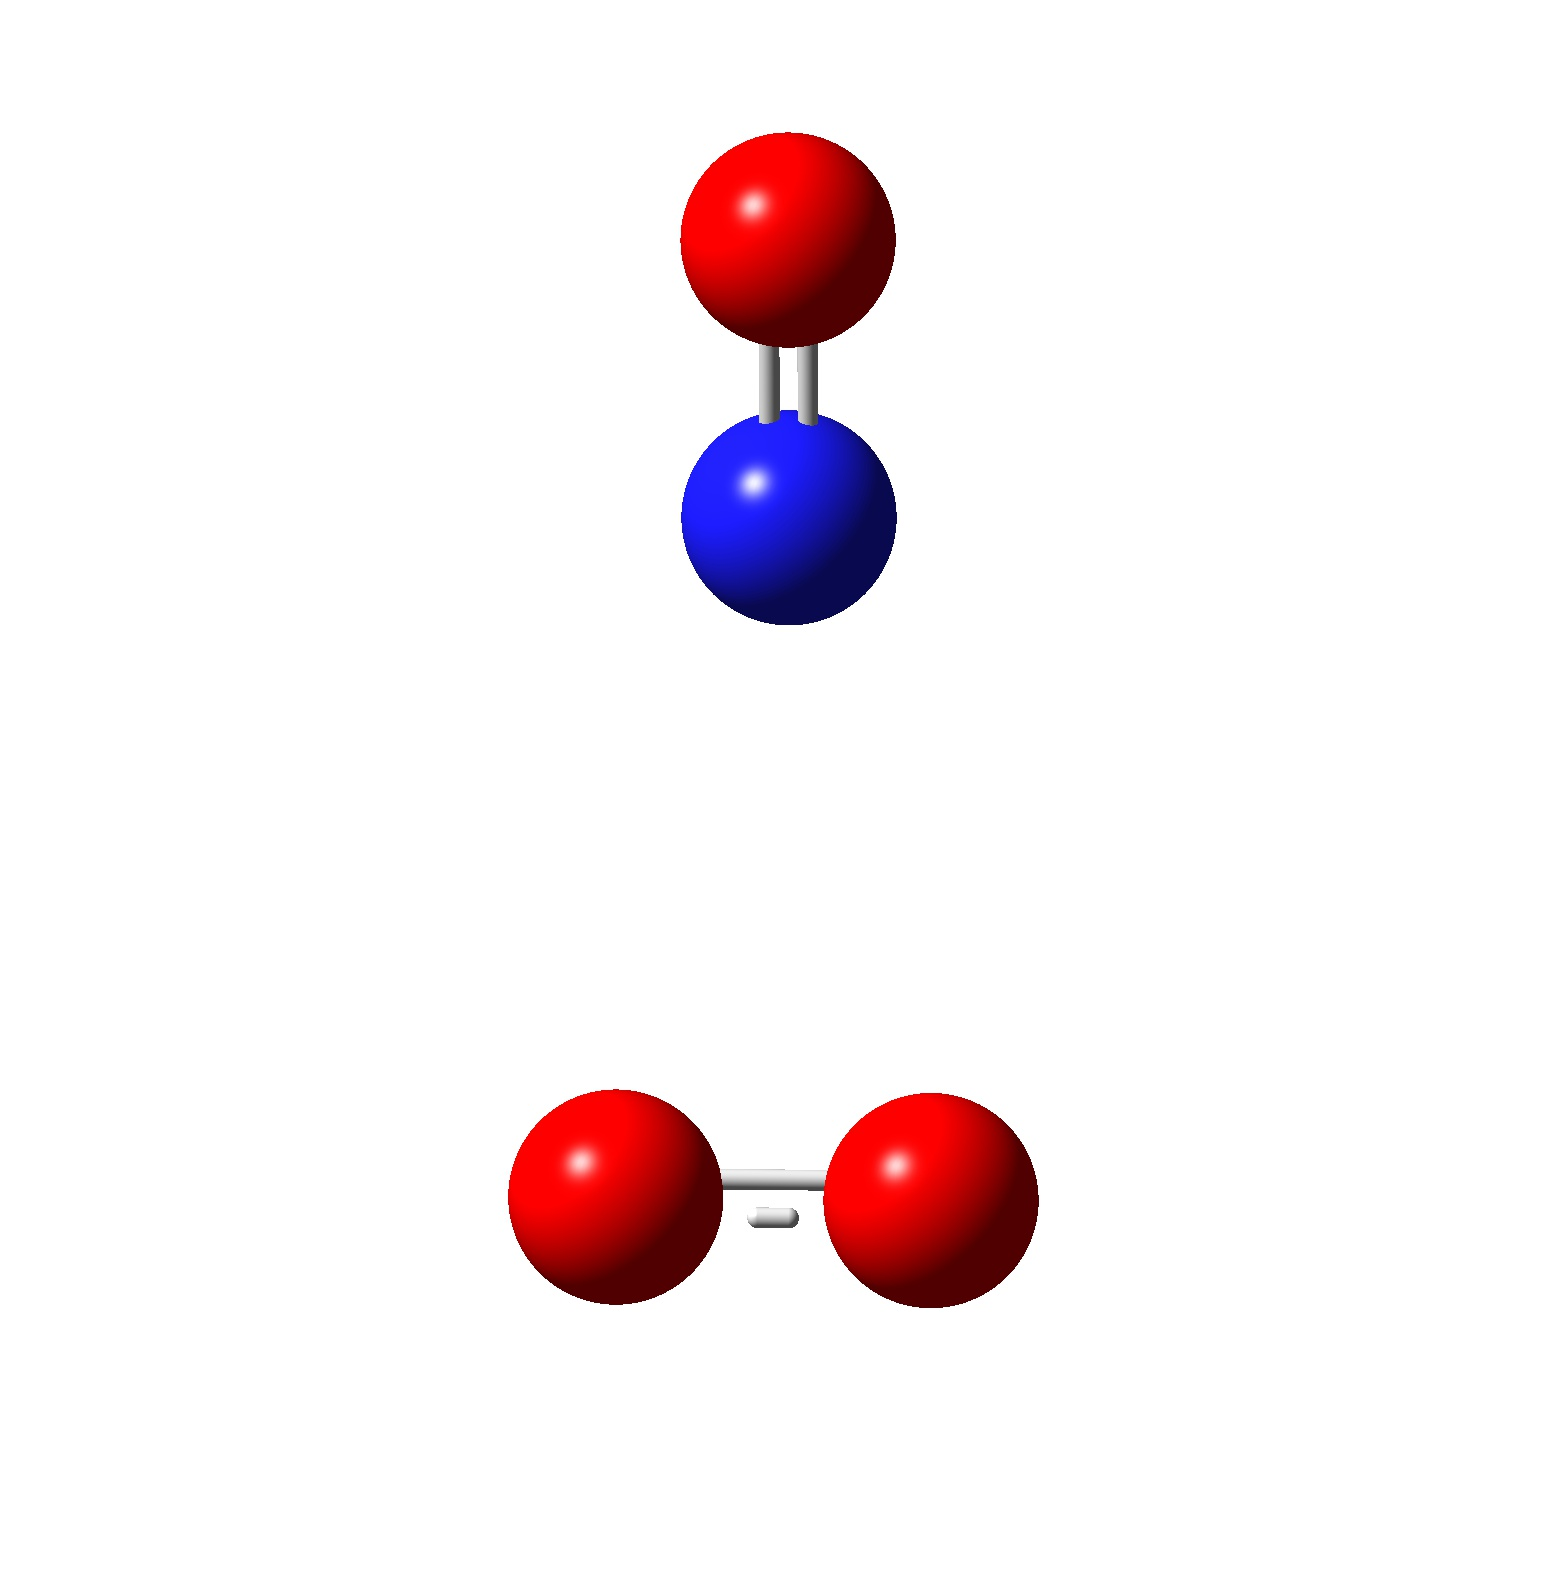}}
  \subfigure[]{\includegraphics[width=0.3\textwidth]{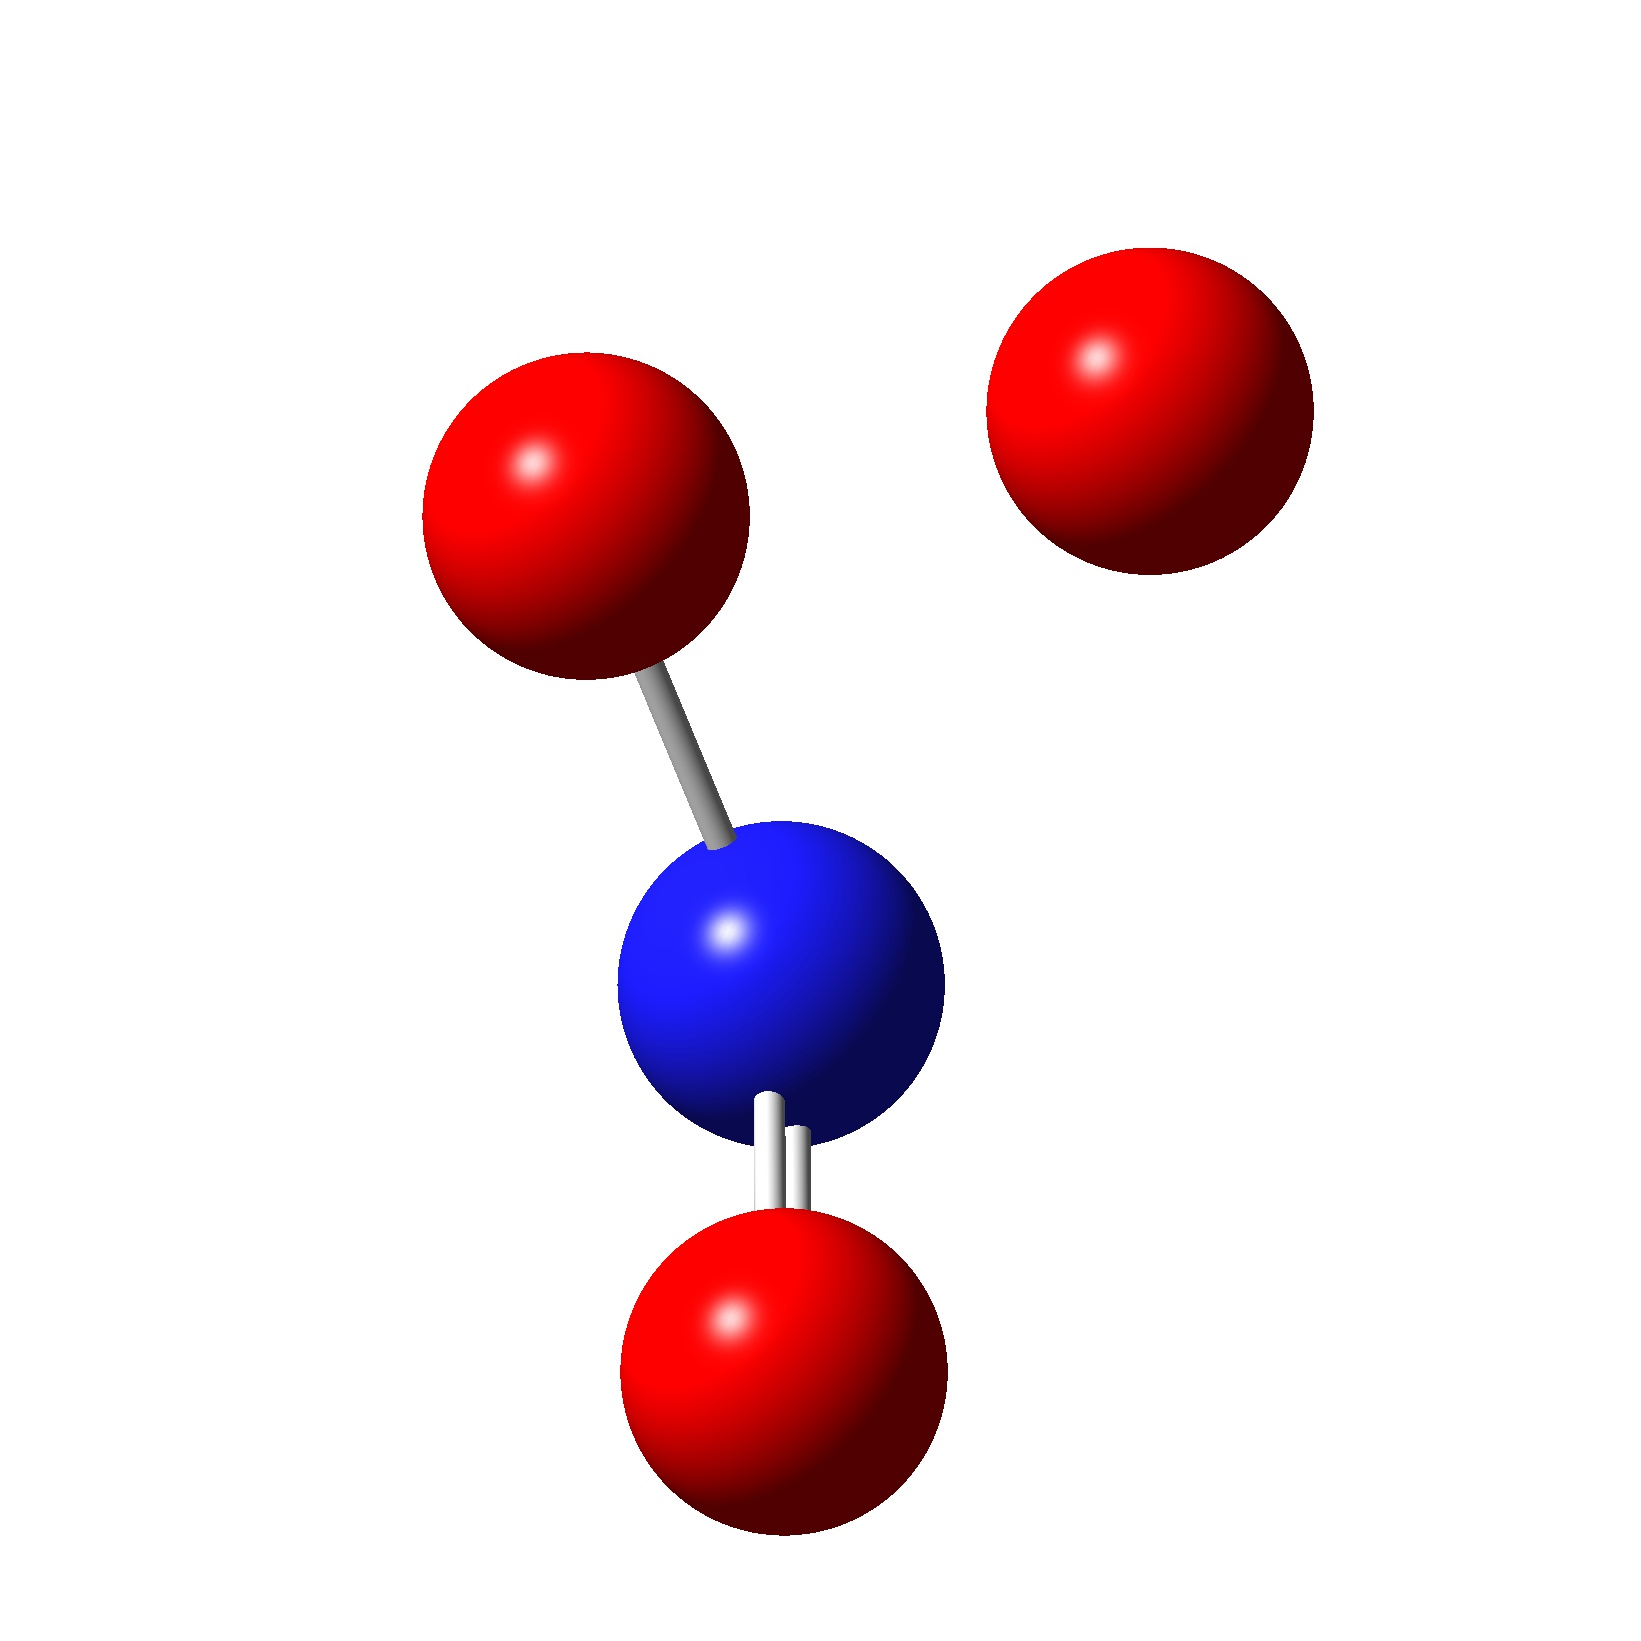}}
  \subfigure[]{\includegraphics[width=0.3\textwidth]{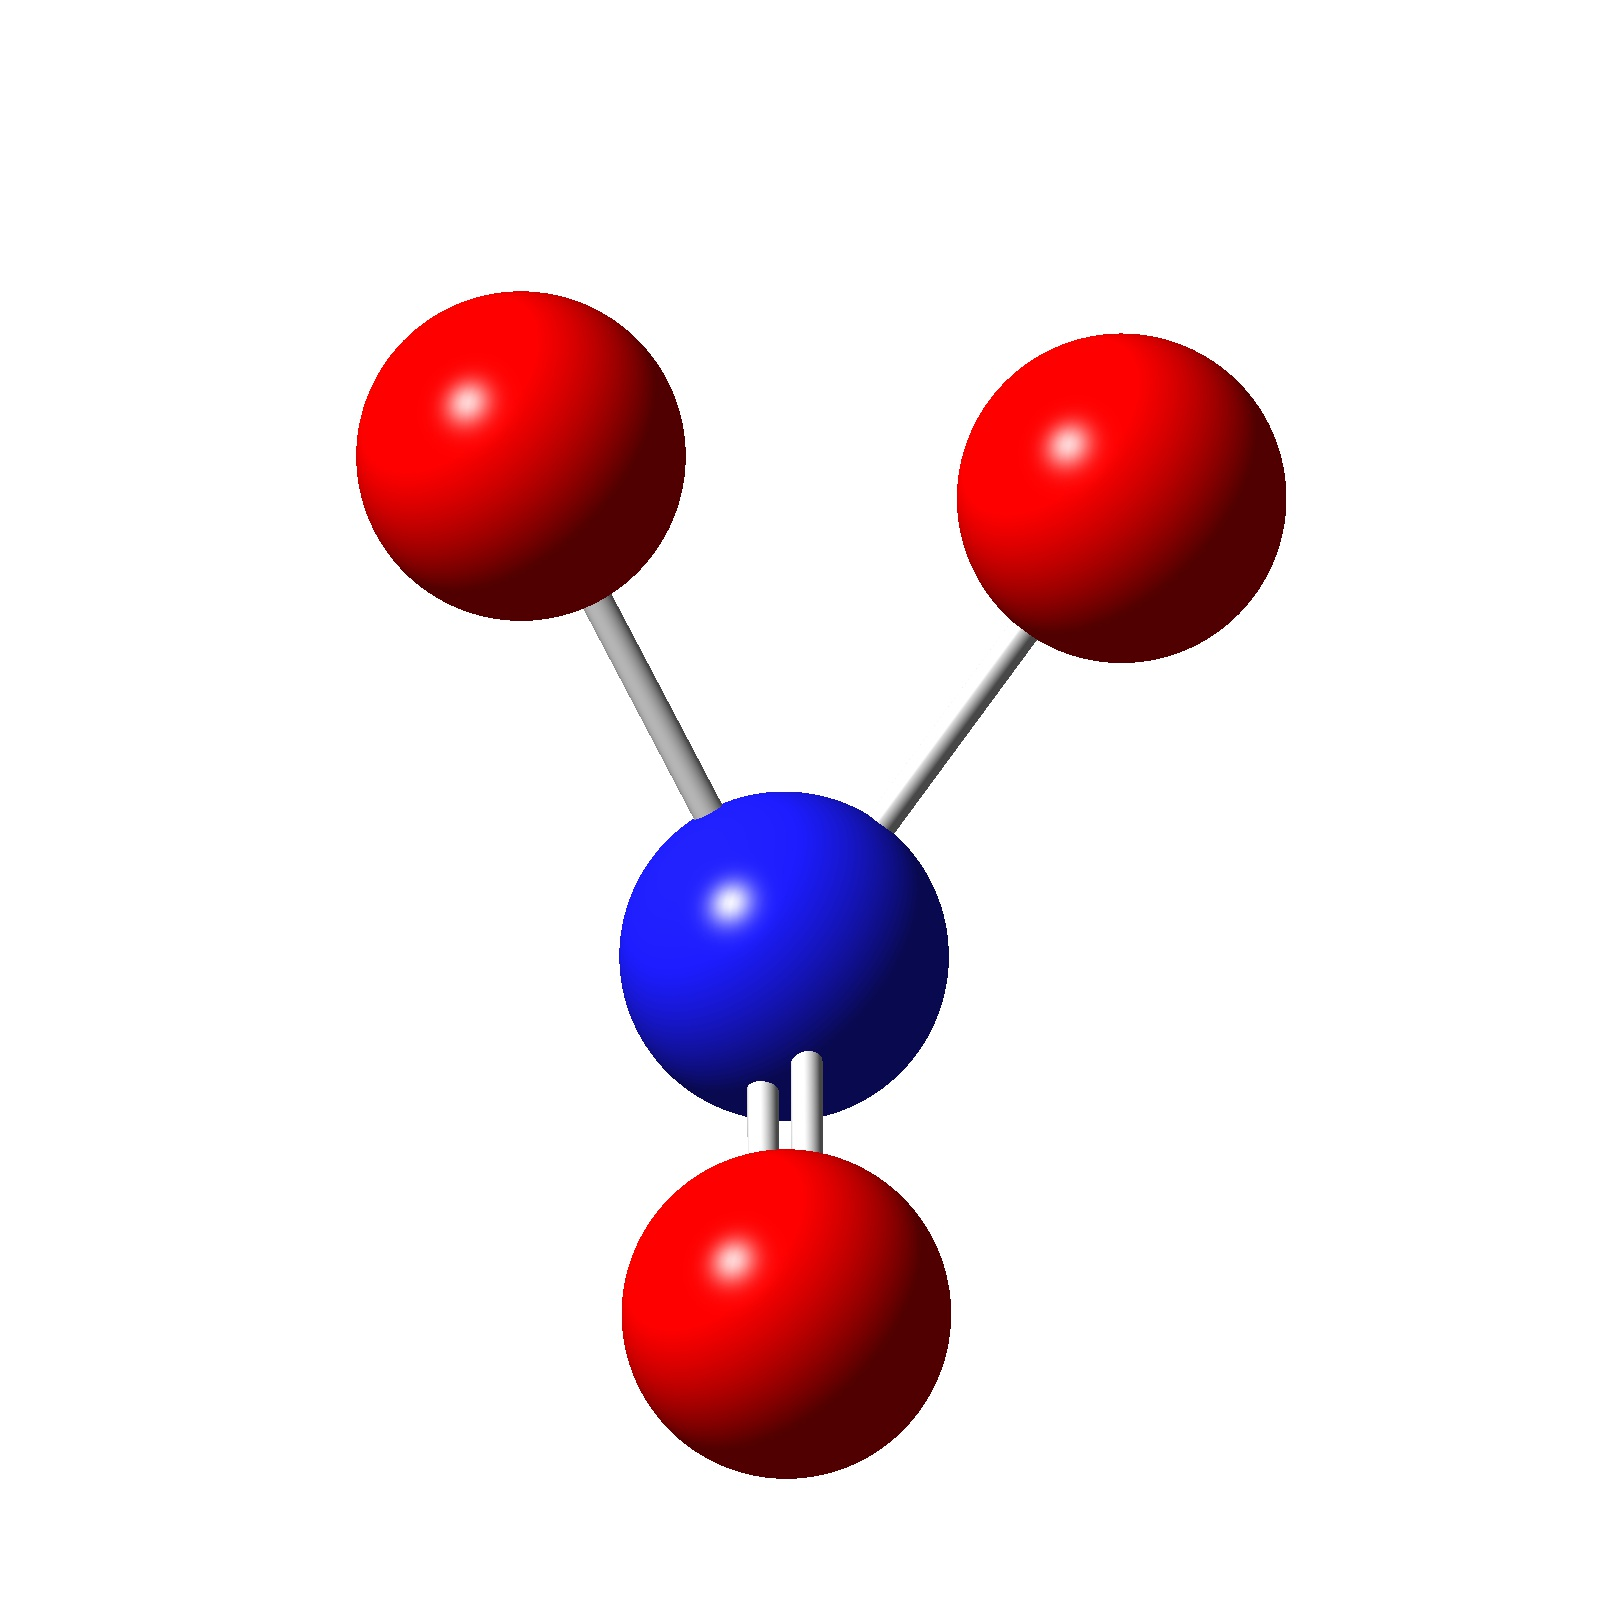}} 
  \subfigure[]{\includegraphics[width=0.3\textwidth]{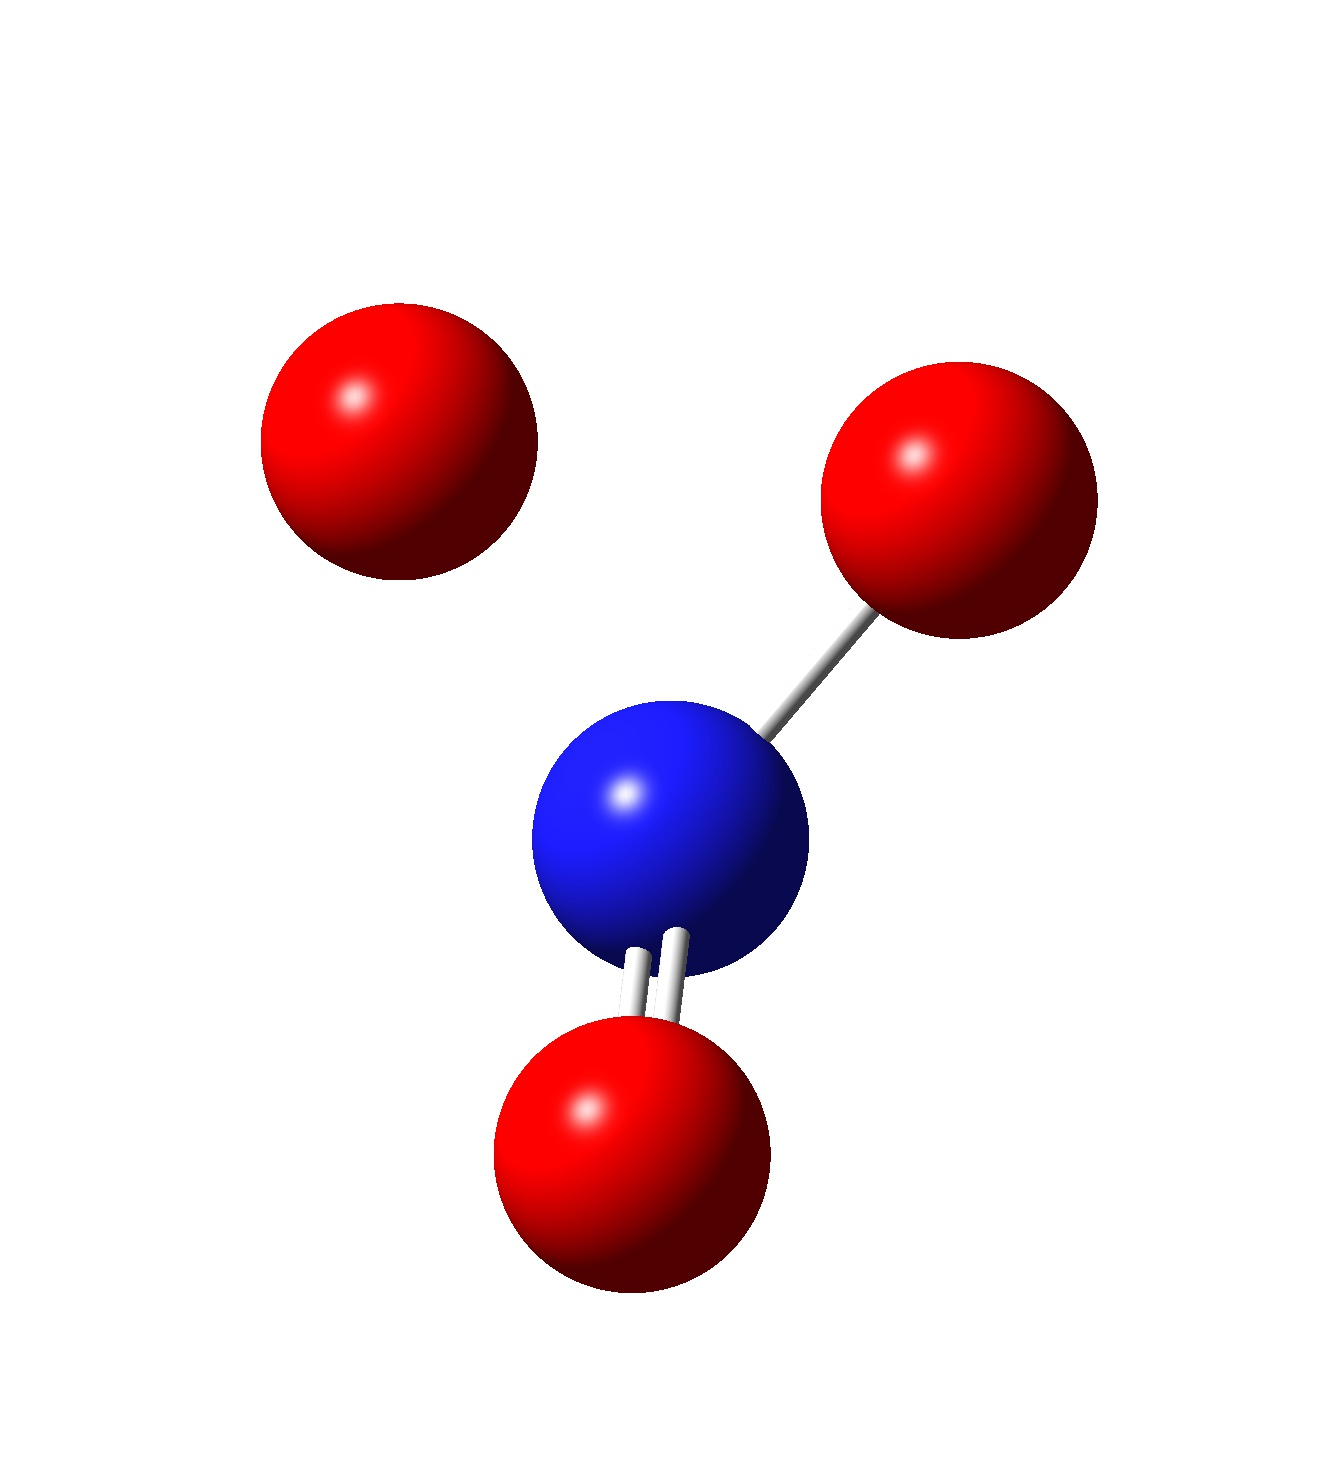}} 
  \subfigure[]{\includegraphics[width=0.3\textwidth]{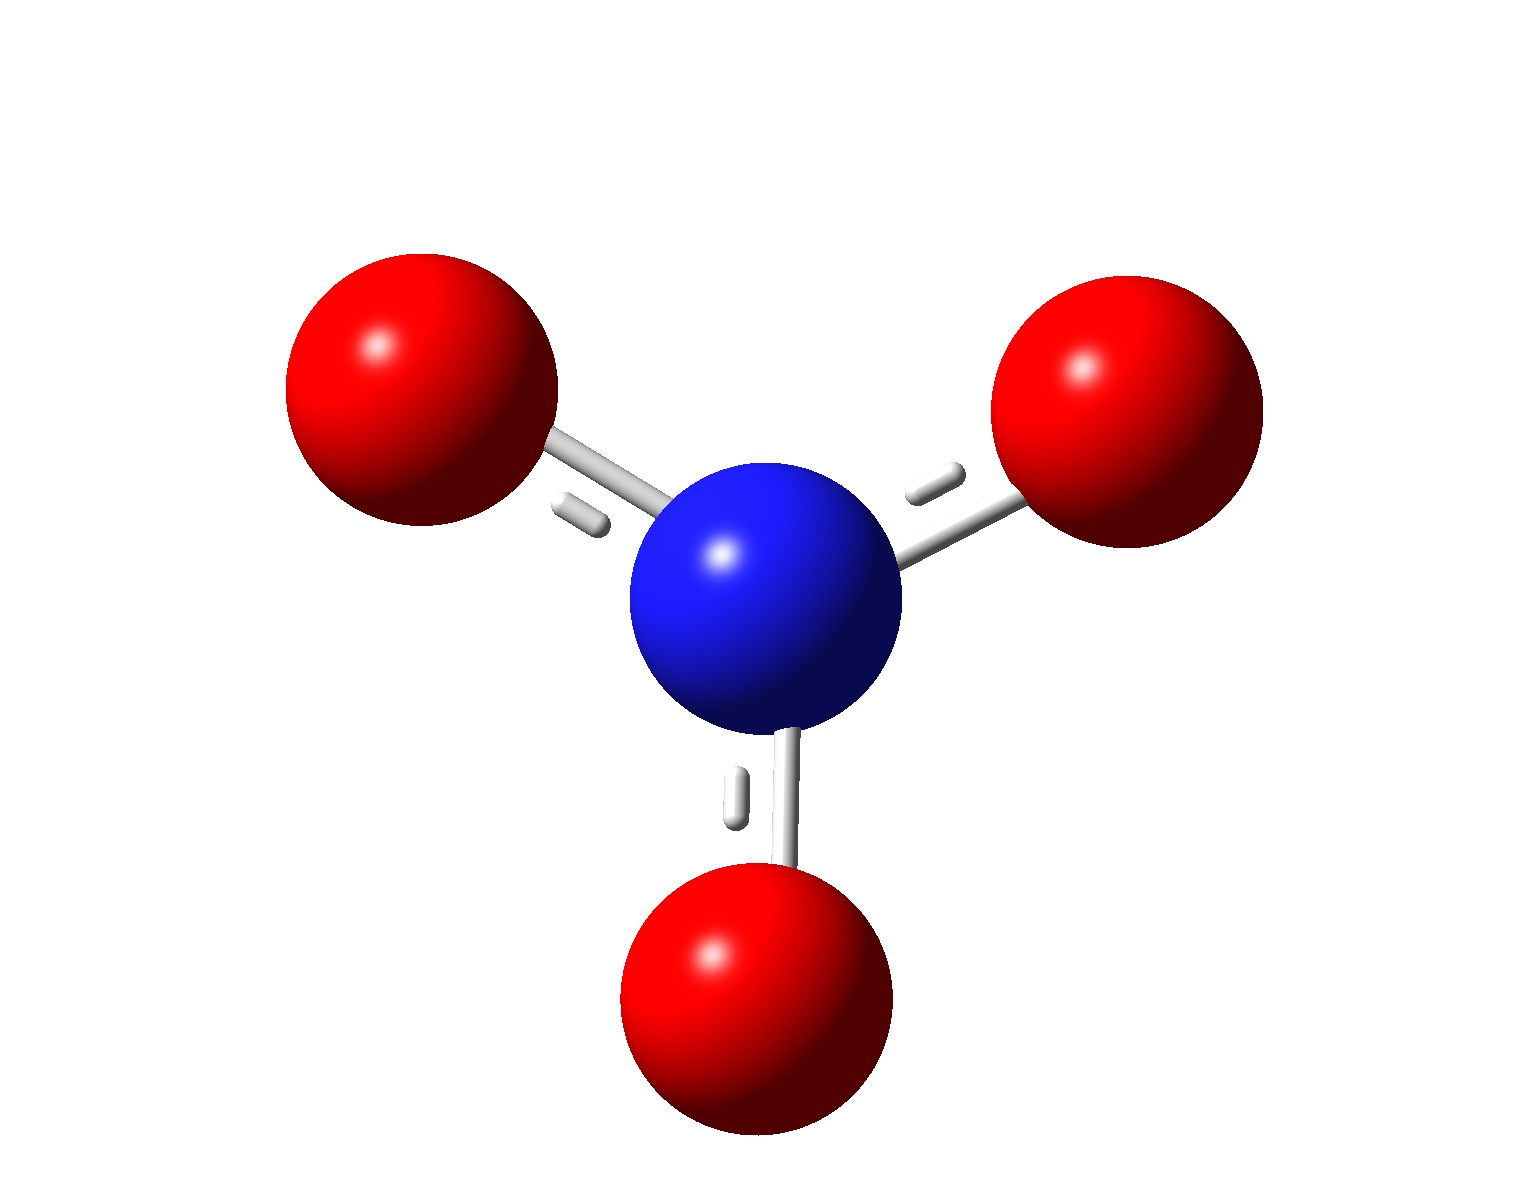}} 
 
  \caption{Optimized structures of (a) O$_{2}$+NO, (b) TS1, (c) INT, (d) TS2, and (e) NO$_{3}$ for step 1 reaction.}
 
\label{SIfig_0}
\end{figure}

For step 2, the IRC for transition state (TS3) (Fig. \ref{SIfig_4}) is calculated, but it does not go to the exact minima unlike in the case of step 1. The exact minima are obtained by optimizing the last points of the IRC of TS3 on both sides. Therefore, the new mass weighted coordinates for the step 2 reaction from the optimized reactant to the final product are calculated from the coordinates collected from the 3D potential energy surface (PES) selecting a reaction path that passes through TS3 (Fig. \ref{SIfig_5}). The potential energy curve from optimized reactant of step 2 to the point where the electronic energy is equal to the sum of the energy of NO$_{3}$ obtained in step 1 and the ground electronic energy of NO at equilibrium bond length is calculated by relax scan (Fig. \ref{SIfig_6}).

\begin{figure}[h]
\centering
  \includegraphics[width=\linewidth]{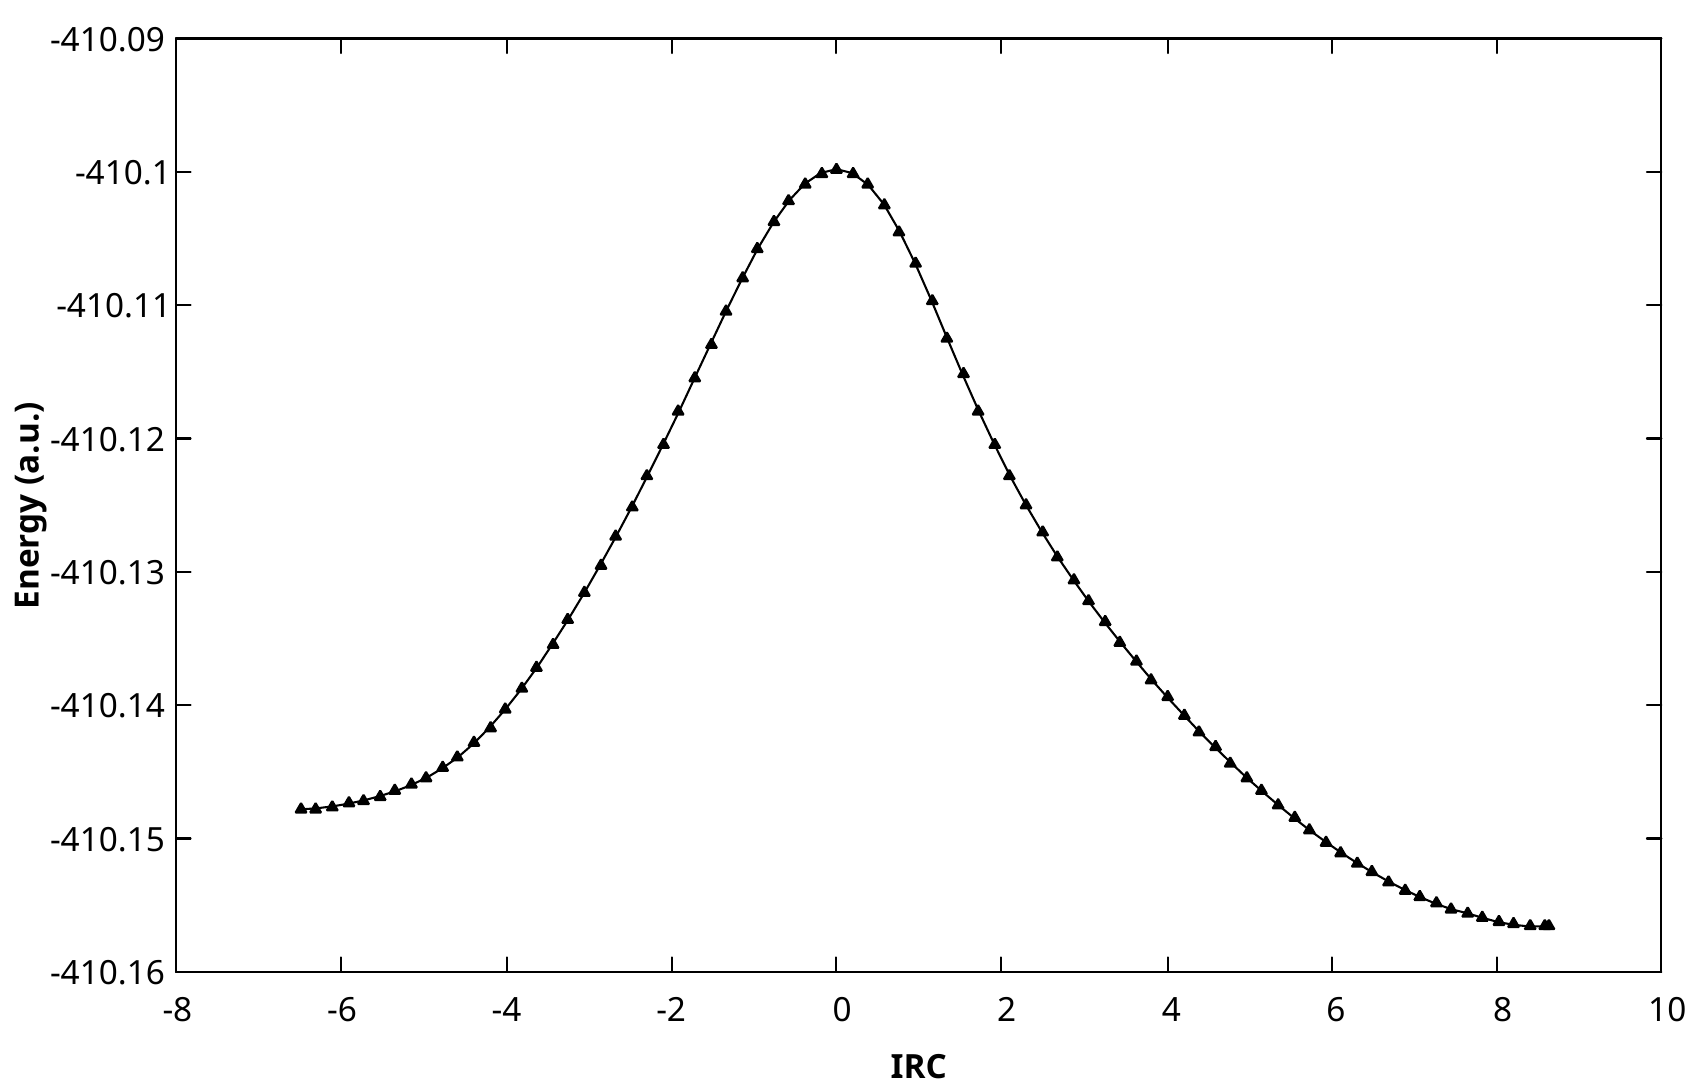}
  \caption{IRC curve for TS3 of step 2 reaction which is showing (from left to right): NO$_{3}$+NO $\rightarrow$ TS3 $\rightarrow$ 2NO$_{2}$}
  \label{SIfig_4}
\end{figure}

\begin{figure}[H]
  \centering
%  \subfigure[]{\includegraphics[width=0.3\textwidth]{prc2.jpg}} 
  \subfigure[]{\includegraphics[width=0.3\textwidth]{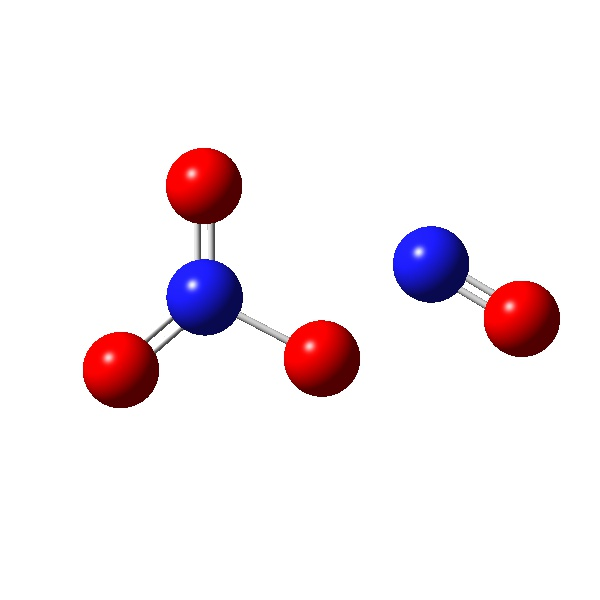}}
  \subfigure[]{\includegraphics[width=0.3\textwidth]{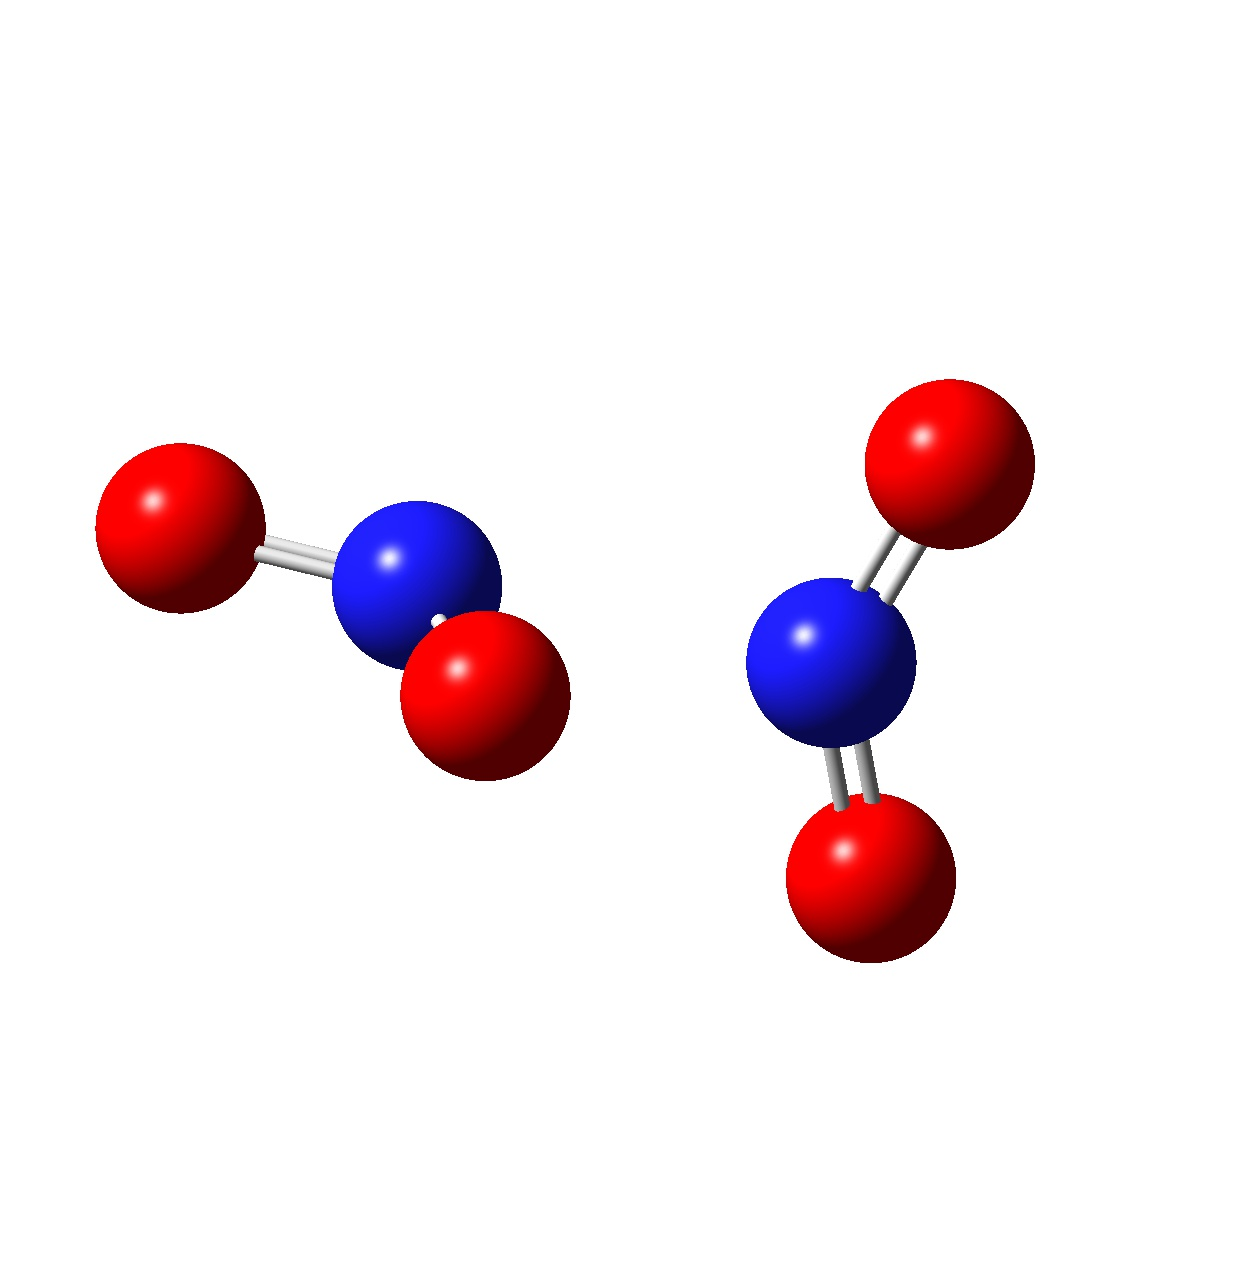}} 
  \subfigure[]{\includegraphics[width=0.3\textwidth]{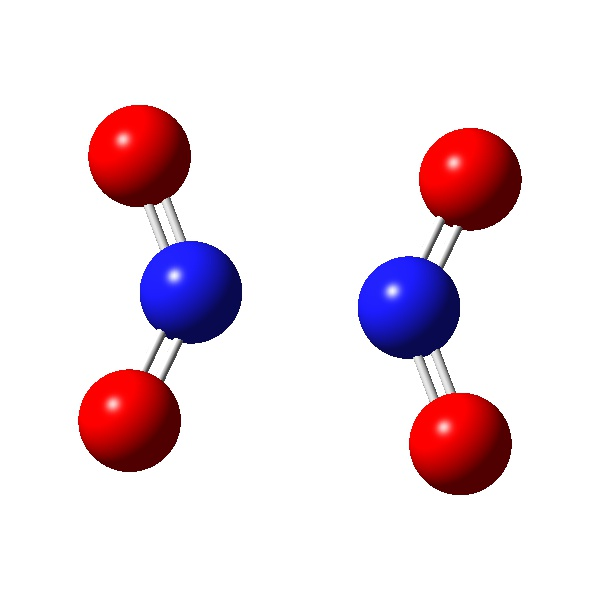}} 
 
  \caption{Optimized structures of (a) NO$_{3}$+NO, (b) TS3, and (c) 2NO$_{2}$ for step 2 reaction.}
 
\label{SIfig_02}
\end{figure}

\begin{figure}[H]
\centering
  \includegraphics[width=\linewidth]{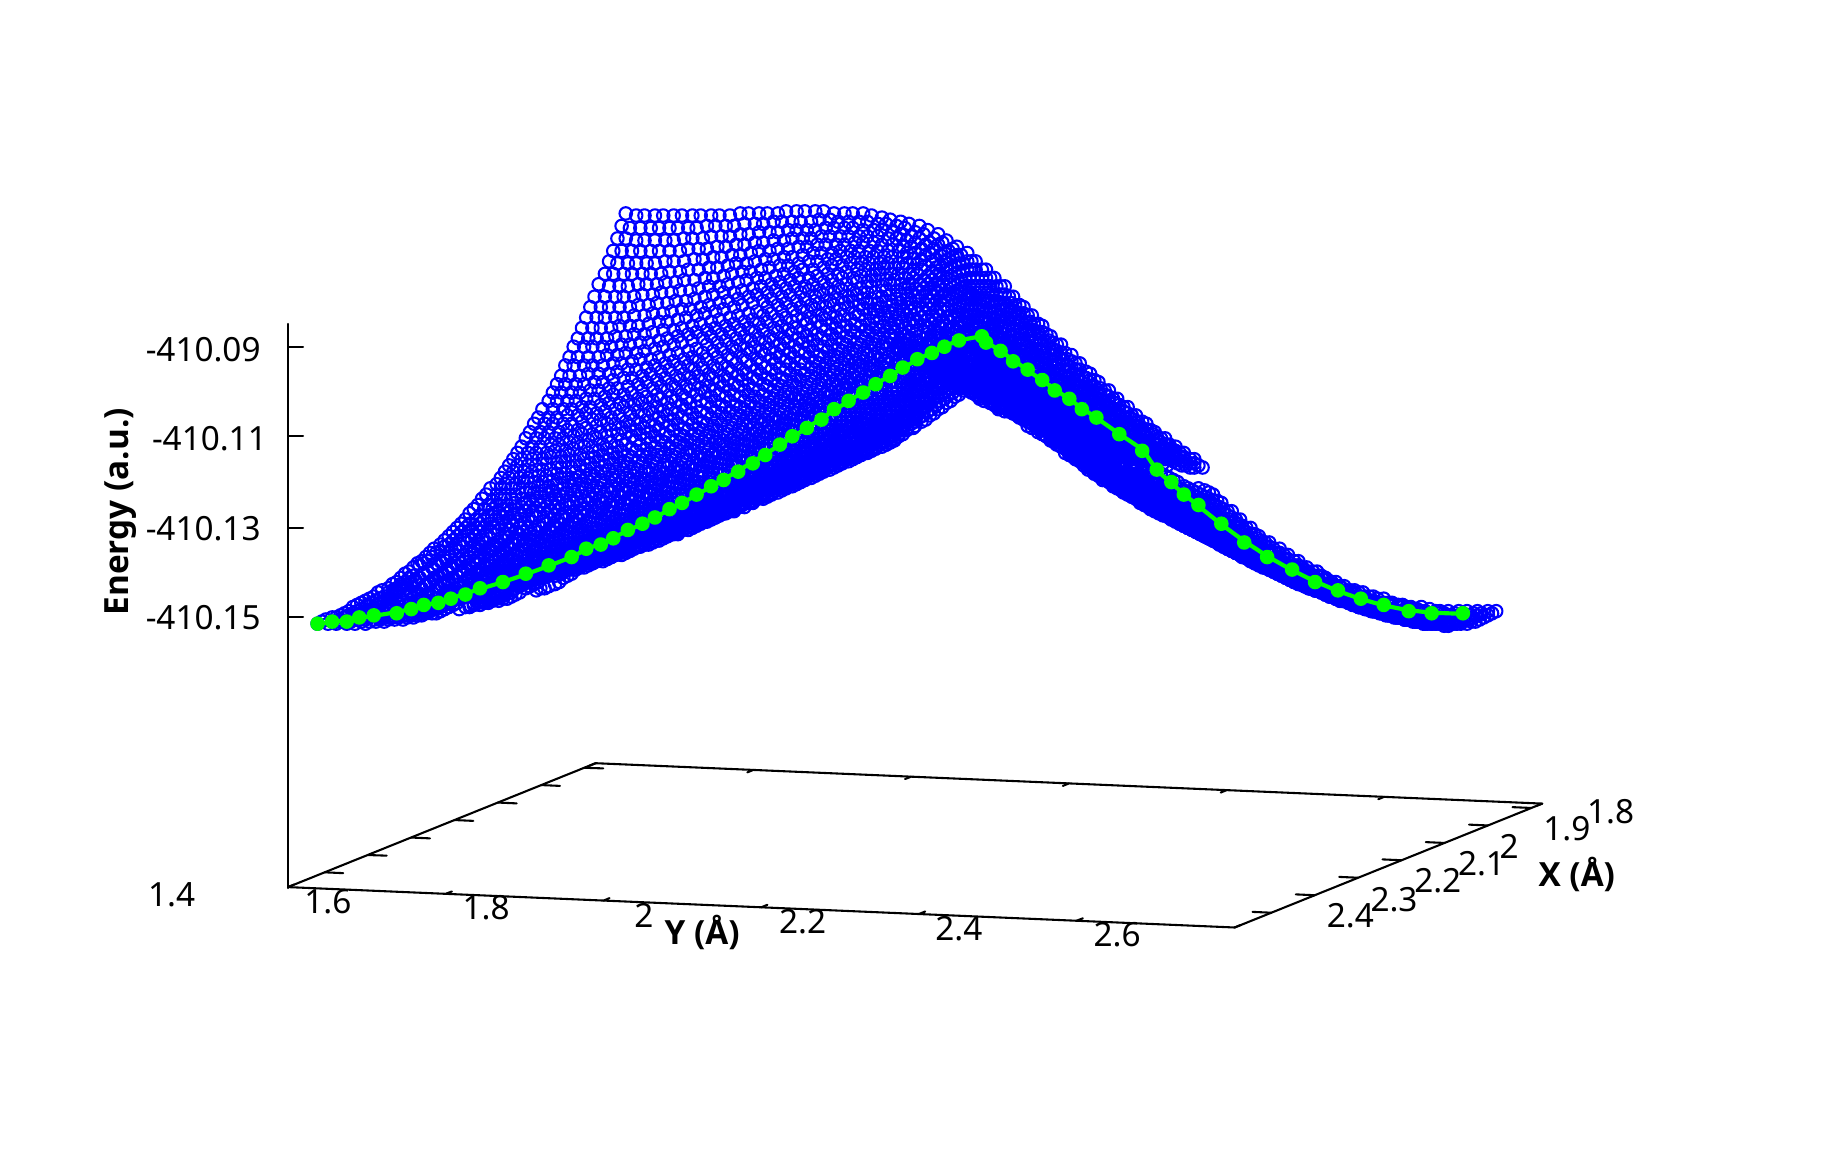}
  \caption{3D potential energy surface of step 2 reaction along with a reaction path from reactant to product (from left to right) which is passing through transition state (TS3) that has been chosen in the calculation.}
  \label{SIfig_5}
\end{figure}

\begin{figure}[H]
\centering
  \includegraphics[width=\linewidth]{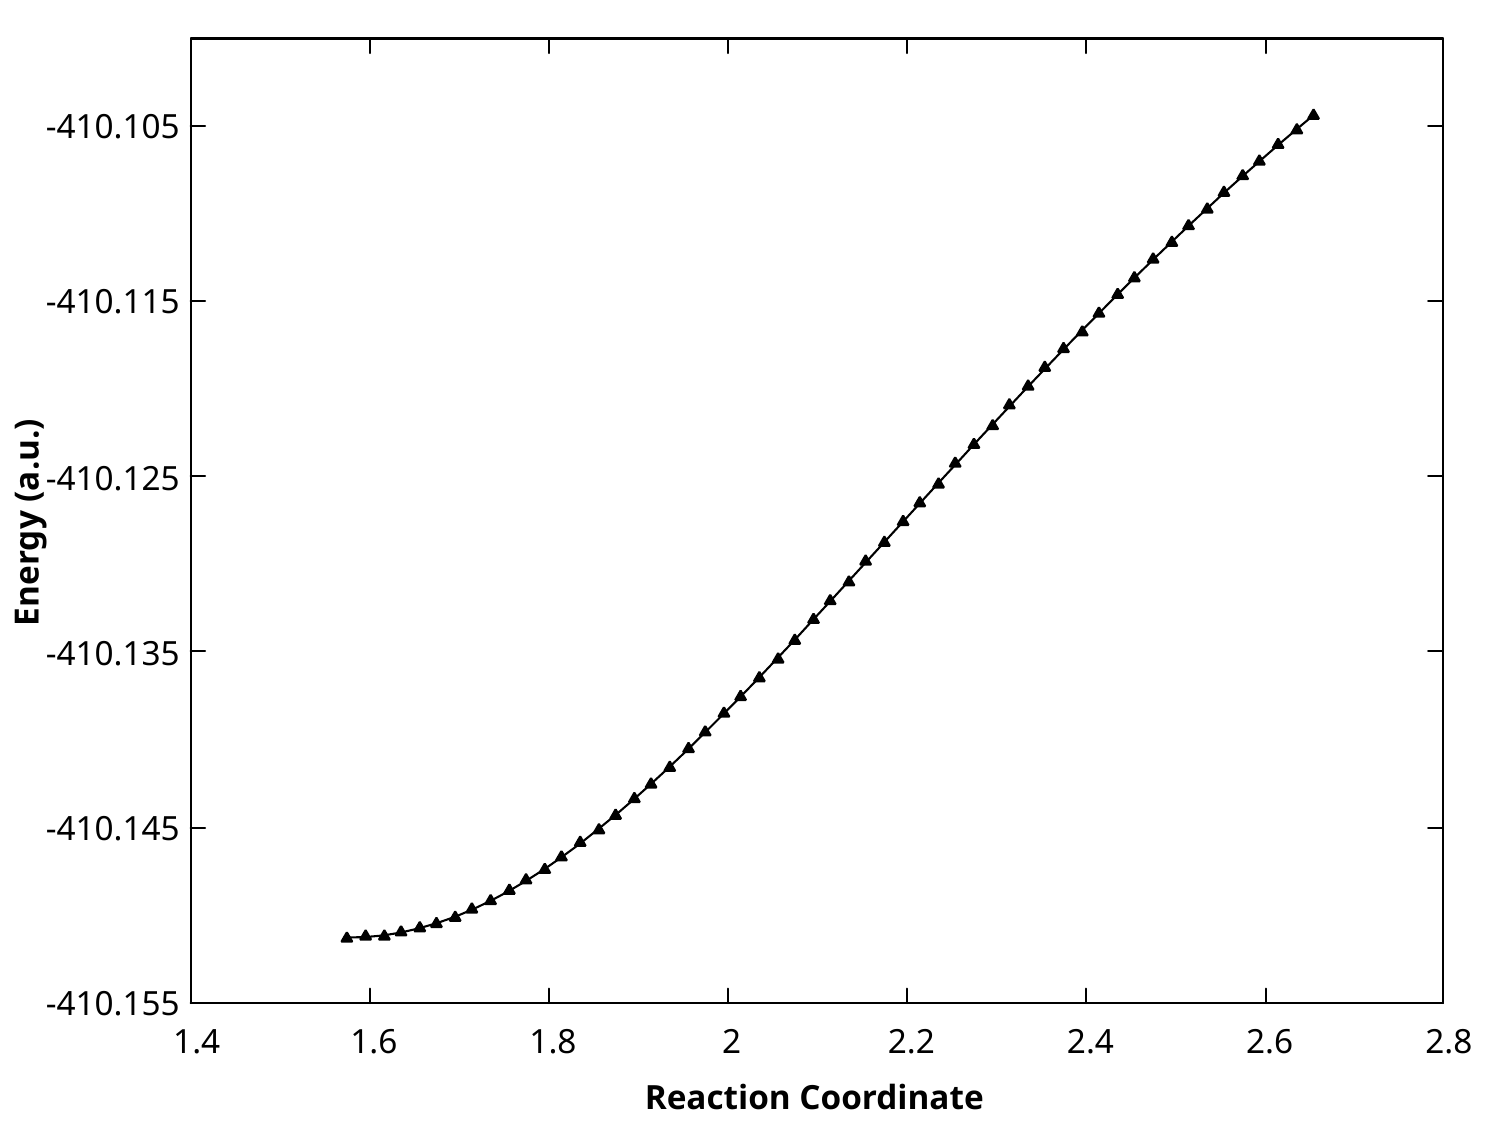}
  \caption{Relax scan to connect potential energy curve of step 2 from reactant to the
point where the energy of reactant complex is equal to the sum of the energy of NO$_{3}$ calculated at step 1 and the ground electronic energy of NO at equilibrium bond length.}
  \label{SIfig_6}
\end{figure}

\begin{figure}[H]
\centering
  \includegraphics[width=\linewidth]{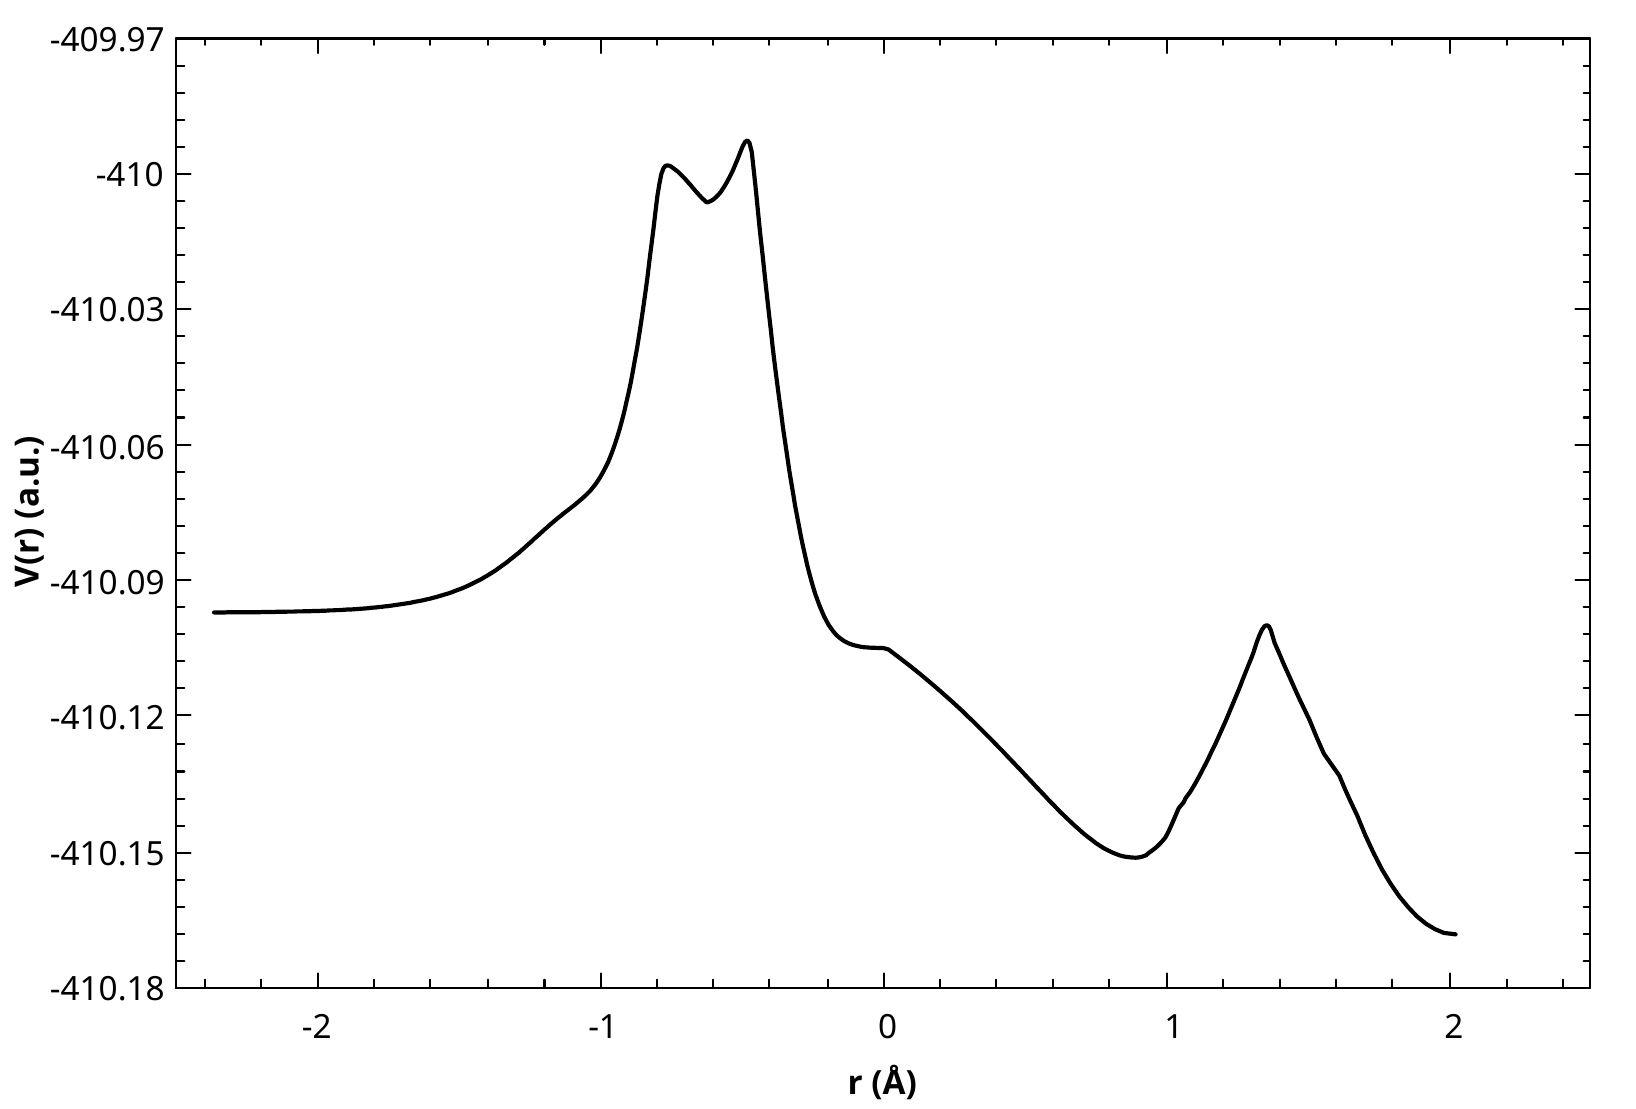}
  \caption{Complete potential energy curve for complete reaction, O$_{2}$+2NO $\rightarrow$ 2NO$_{2}$ by connecting the potential energy curves of steps 1 and 2 using mass weighted coordinate r.}
  \label{SIfig_7}
\end{figure}

\begin{figure}[H]
\centering
  \includegraphics[width=\linewidth]{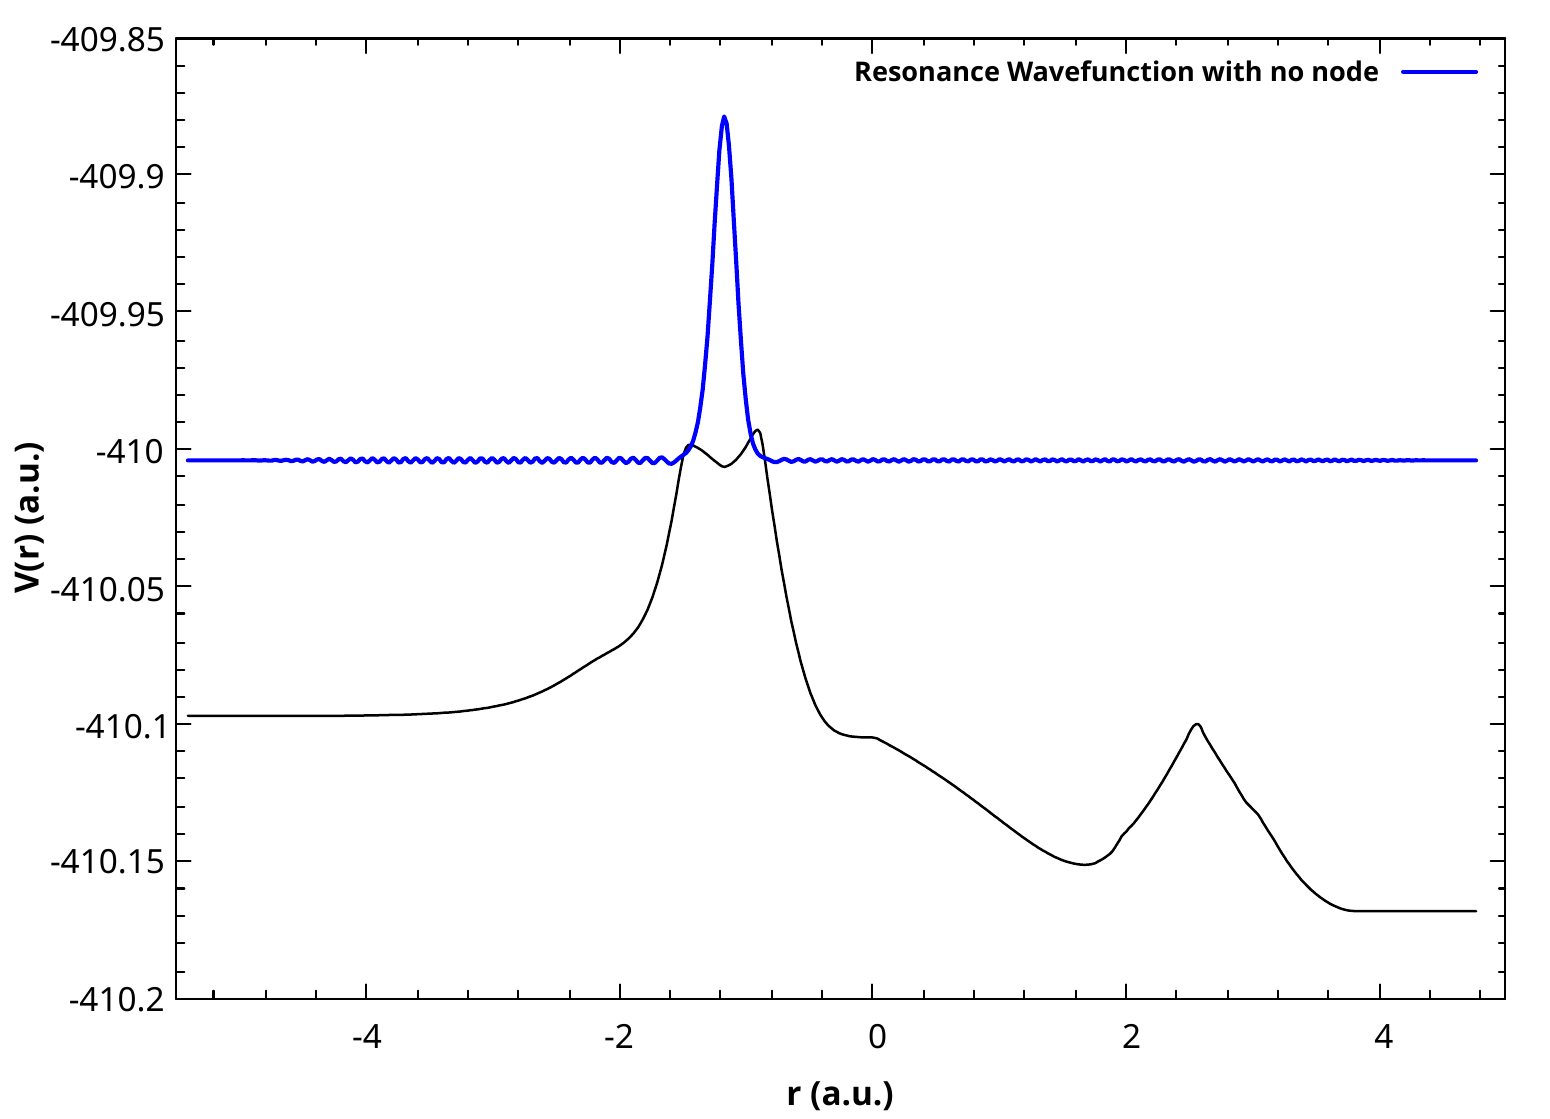}
  \caption{Resonance wave function having no node superimposed on potential. This wave function is calculated at $\theta$ = 0.14 radian which is the stationary point of the resonance $\theta$-trajectories.}
  \label{SIfig_8}
\end{figure}

\begin{figure}[H]
\centering
  \includegraphics[width=\linewidth]{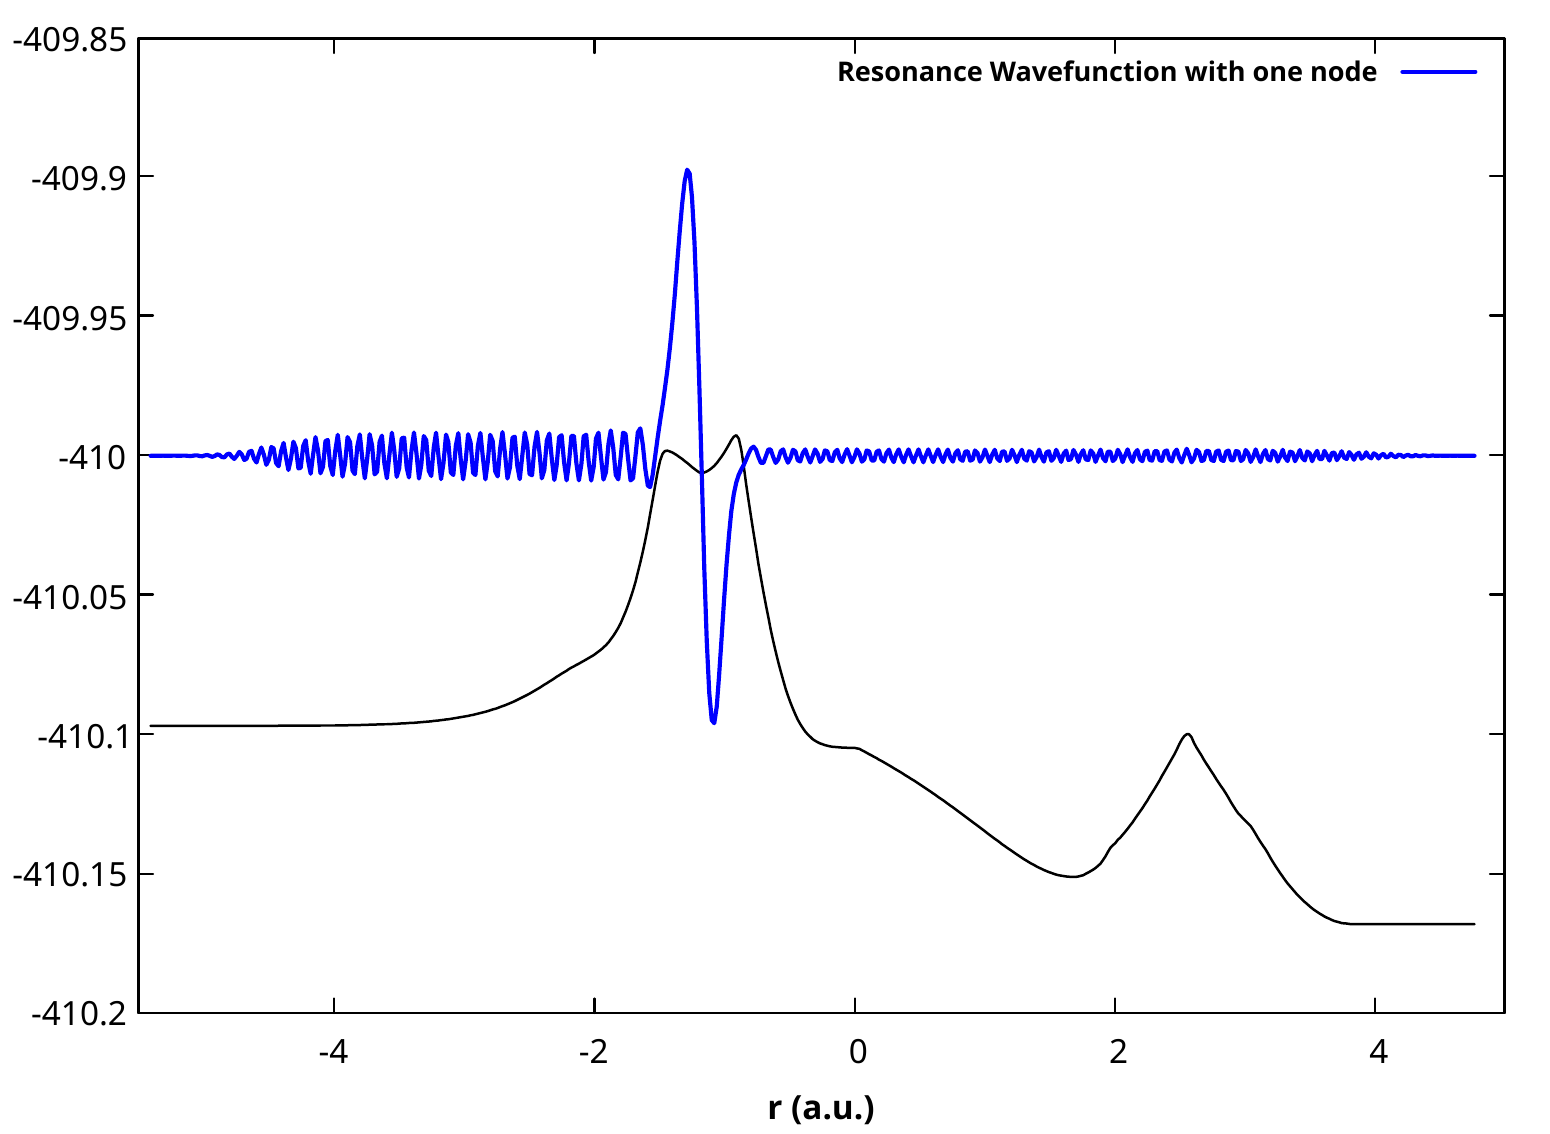}
  \caption{Resonance wave function having one node superimposed on potential. This wave function is calculated at $\theta$ = 0.14 radian which is the stationary point of the resonance $\theta$-trajectories.}
  \label{SIfig_9}
\end{figure}

\begin{figure}[H]
\centering
  \includegraphics[width=\linewidth]{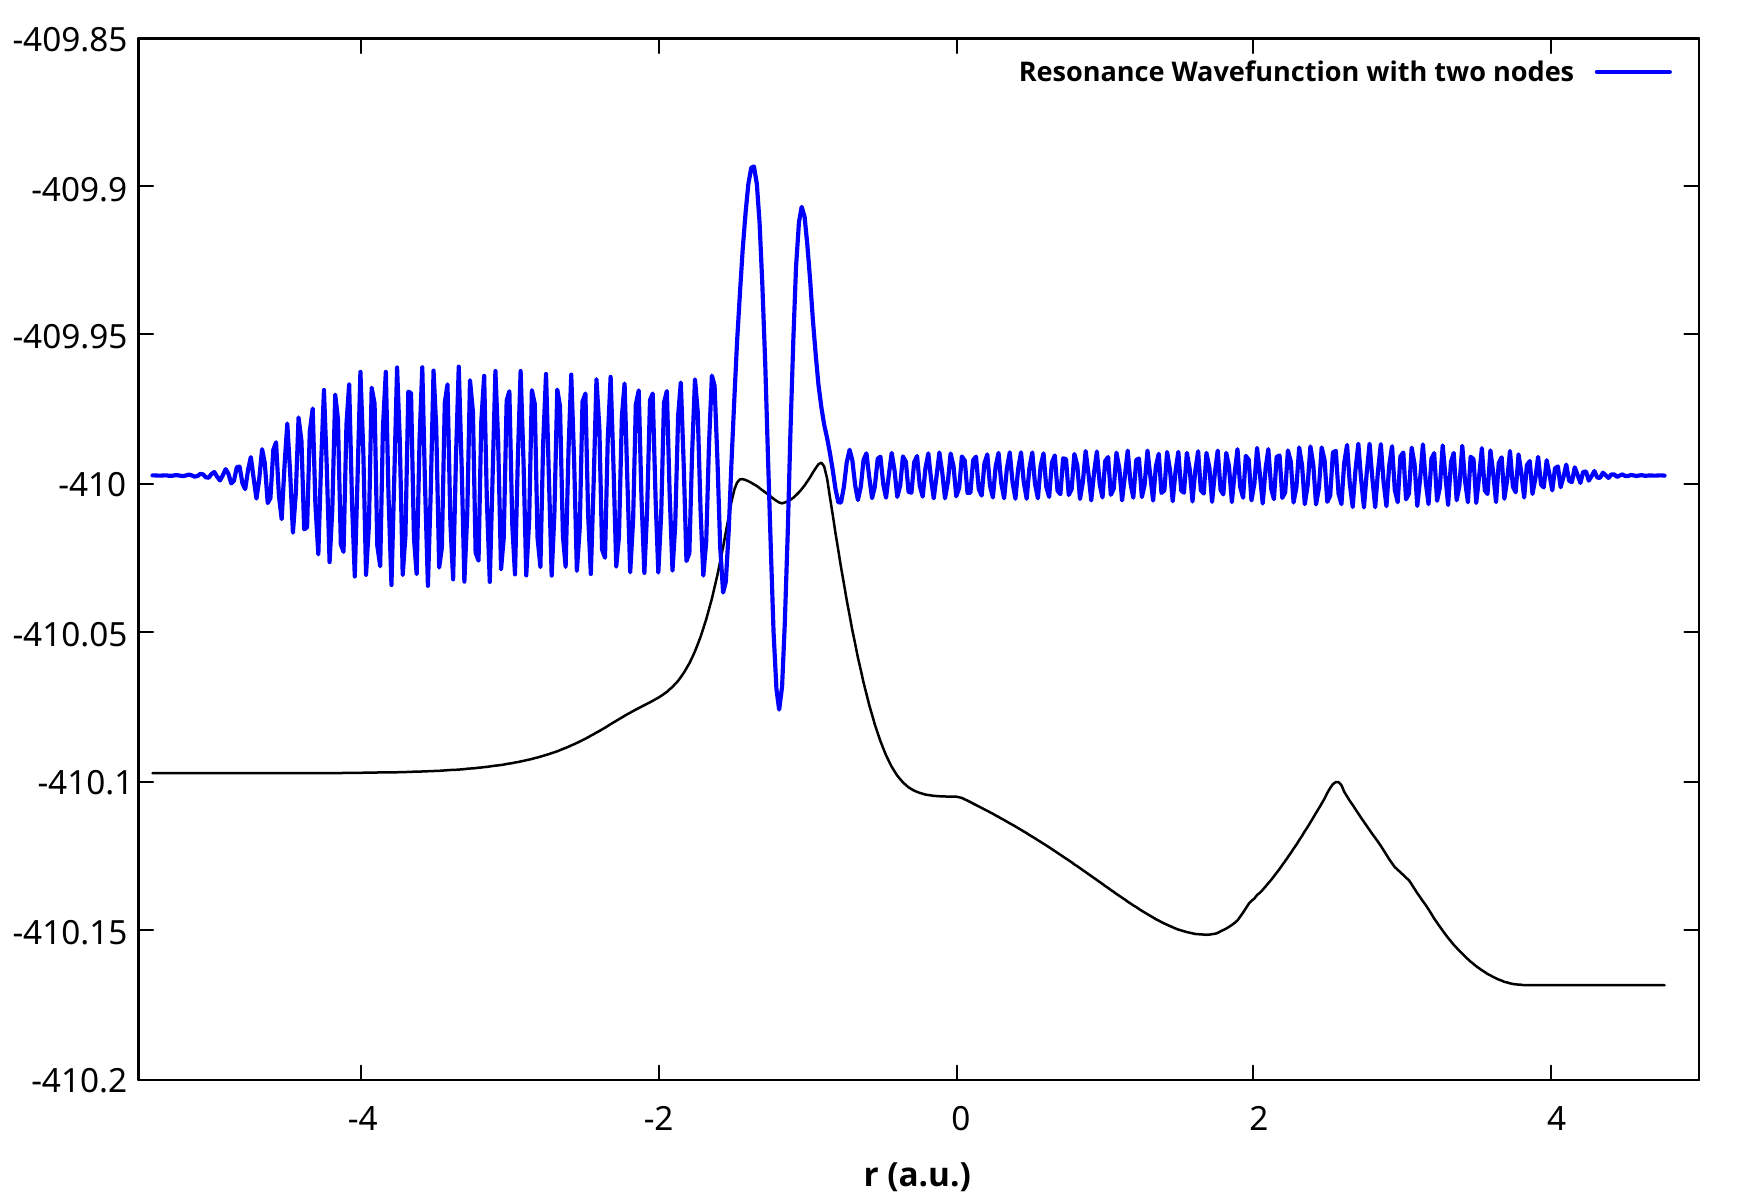}
  \caption{Resonance wave function having two nodes superimposed on potential. This wave function is calculated at $\theta$ = 0.14 radian which is the stationary point of the resonance $\theta$-trajectories.}
  \label{SIfig_10}
\end{figure}

\begin{figure}[H]
\centering
  \includegraphics[width=\linewidth]{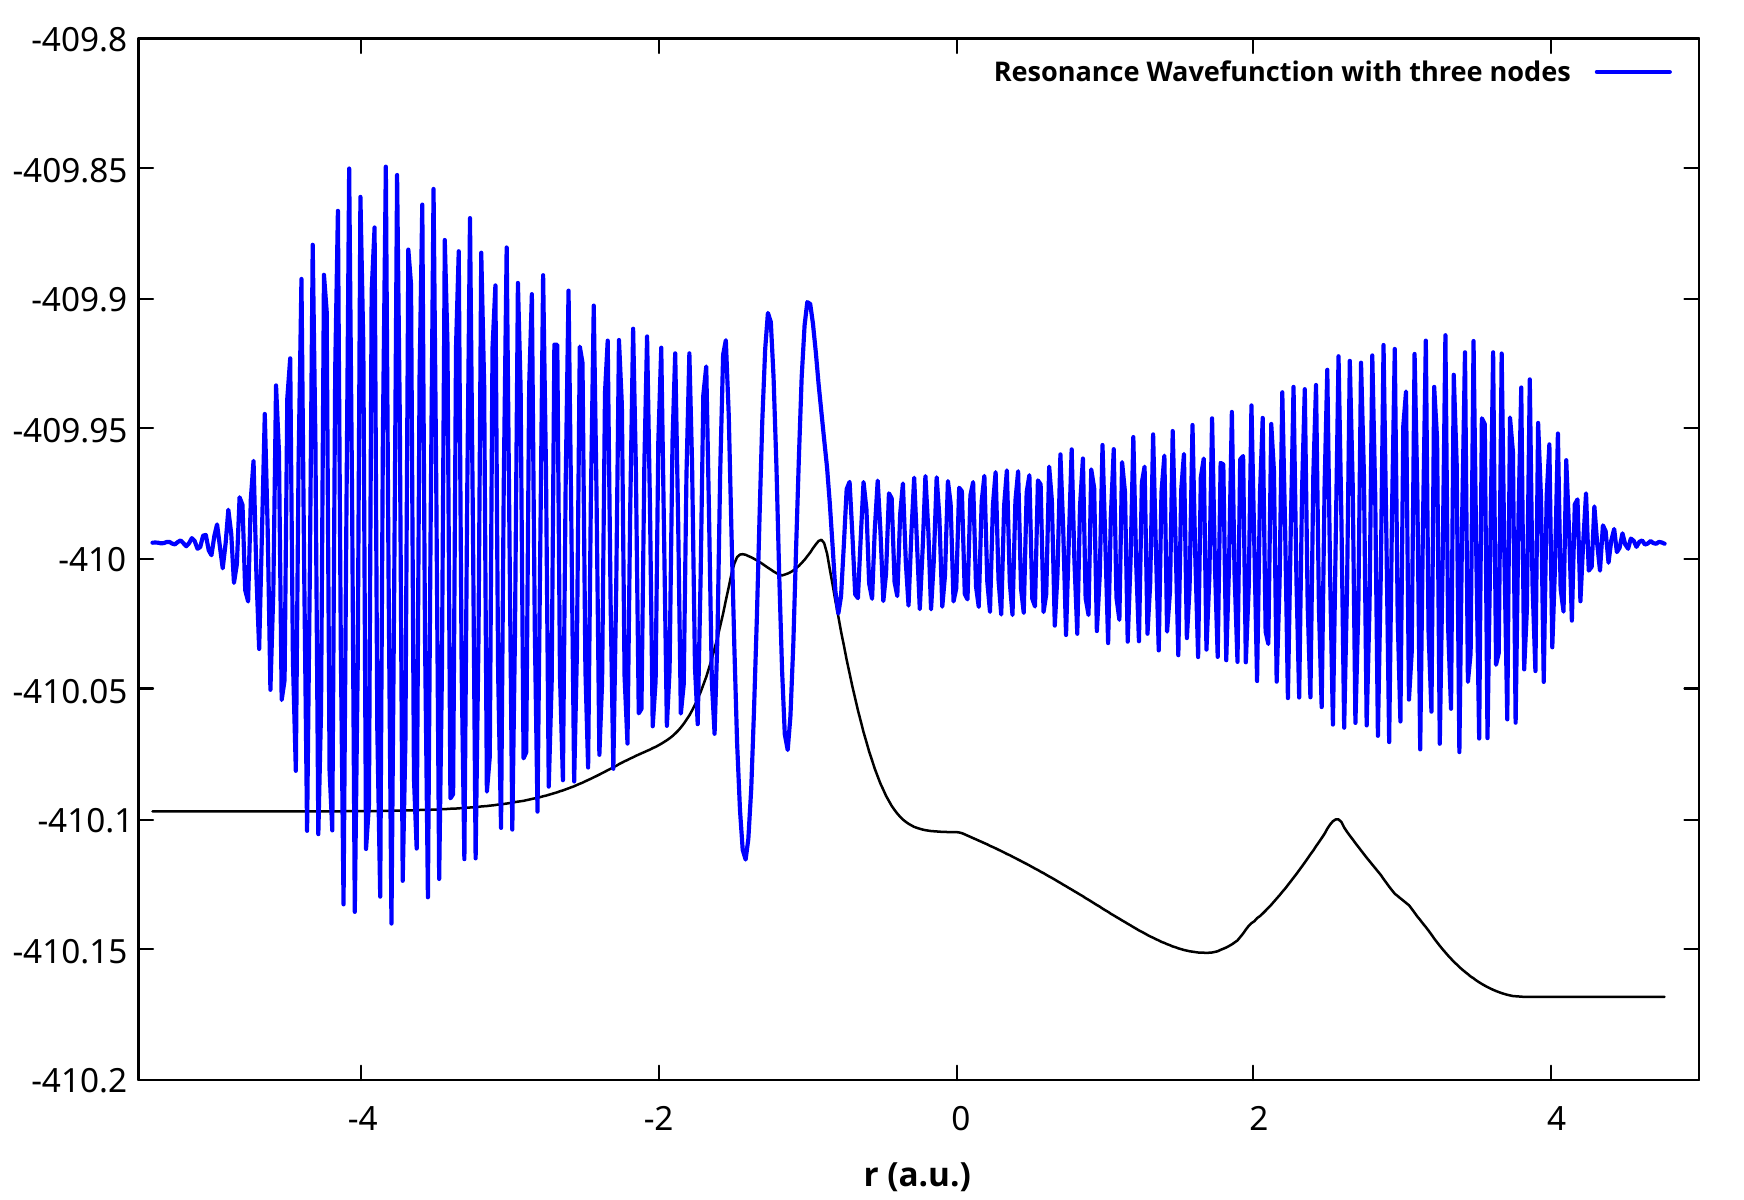}
  \caption{Resonance wave function having three nodes superimposed on potential. This wave function is calculated at $\theta$ = 0.14 radian which is the stationary point of the resonance $\theta$-trajectories.}
  \label{SIfig_11}
\end{figure}

\begin{figure}[H]
\centering
  \includegraphics[width=\linewidth]{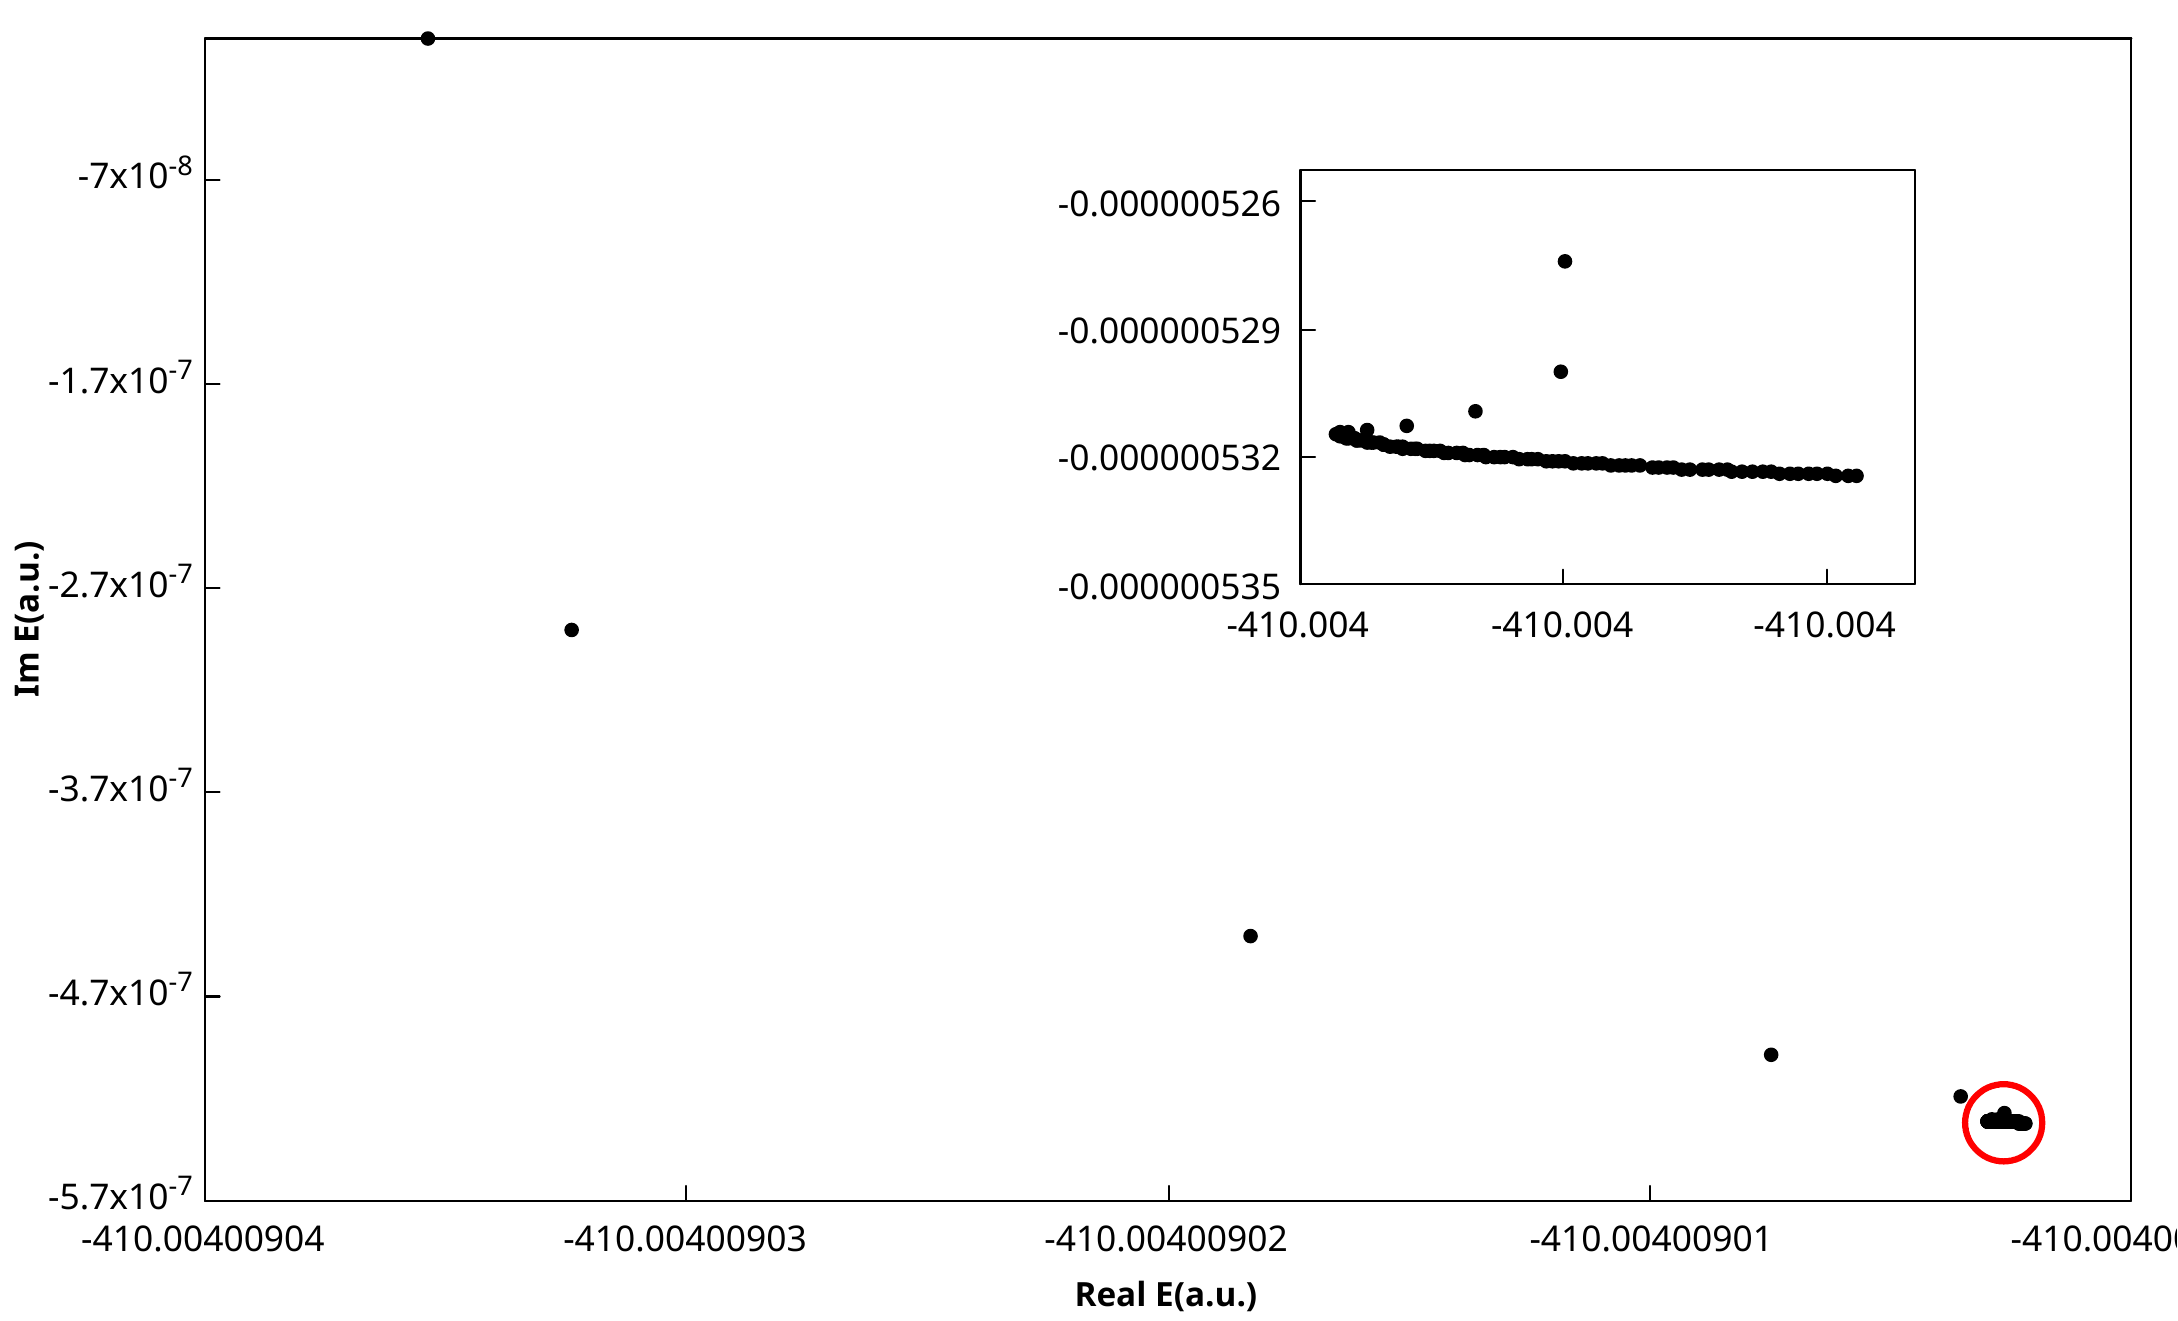}
  \caption{$\theta$-trajectory of resonance with no node . The circled potion is zoomed in for clarity.}
  \label{SIfig_12}
\end{figure}

\begin{figure}[H]
\centering
  \includegraphics[width=\linewidth]{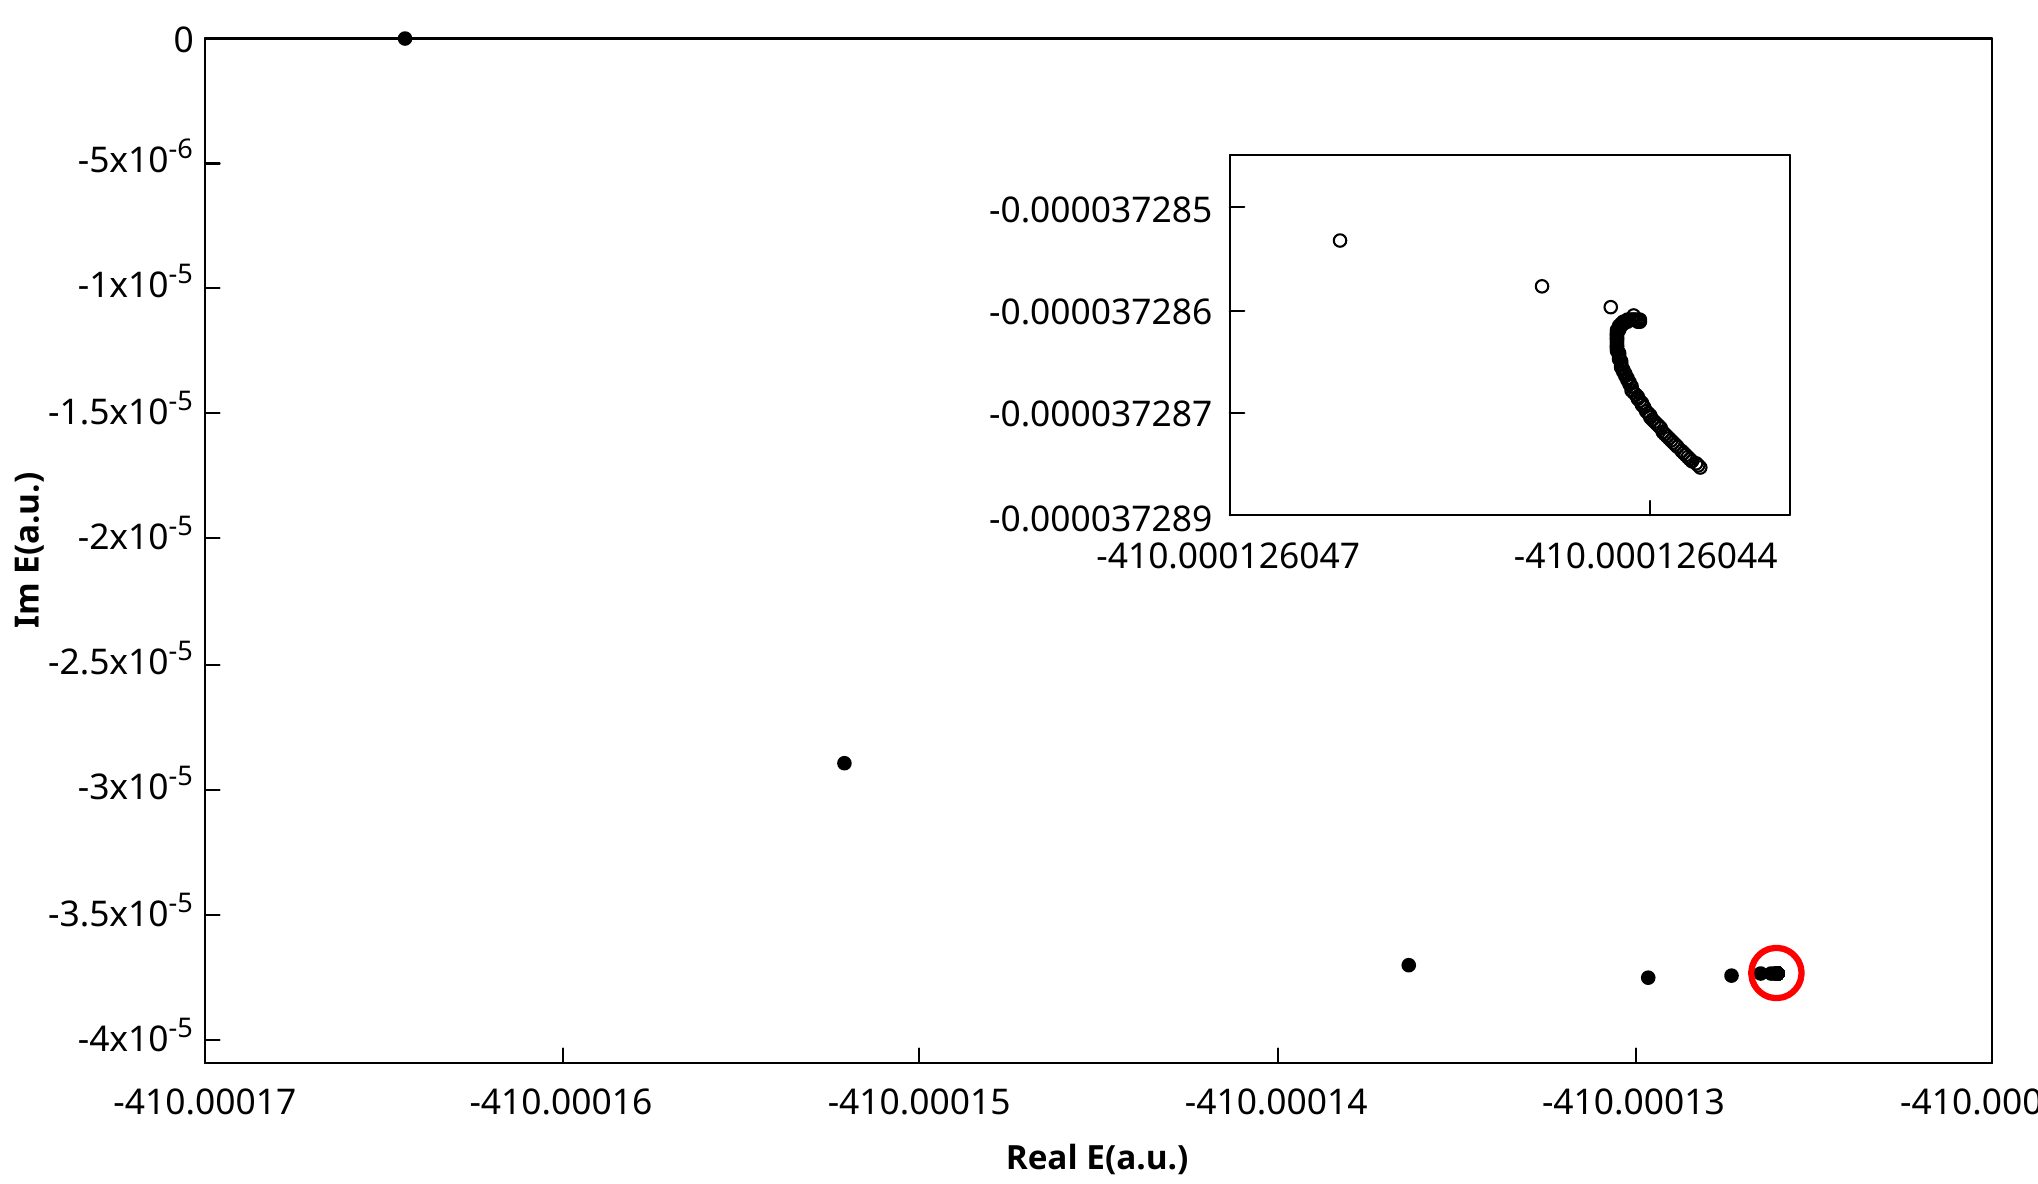}
  \caption{$\theta$-trajectory of resonance withone node. The circled potion is zoomed in for clarity.}
  \label{SIfig_13}
\end{figure}

\begin{figure}[H]
\centering
  \includegraphics[width=\linewidth]{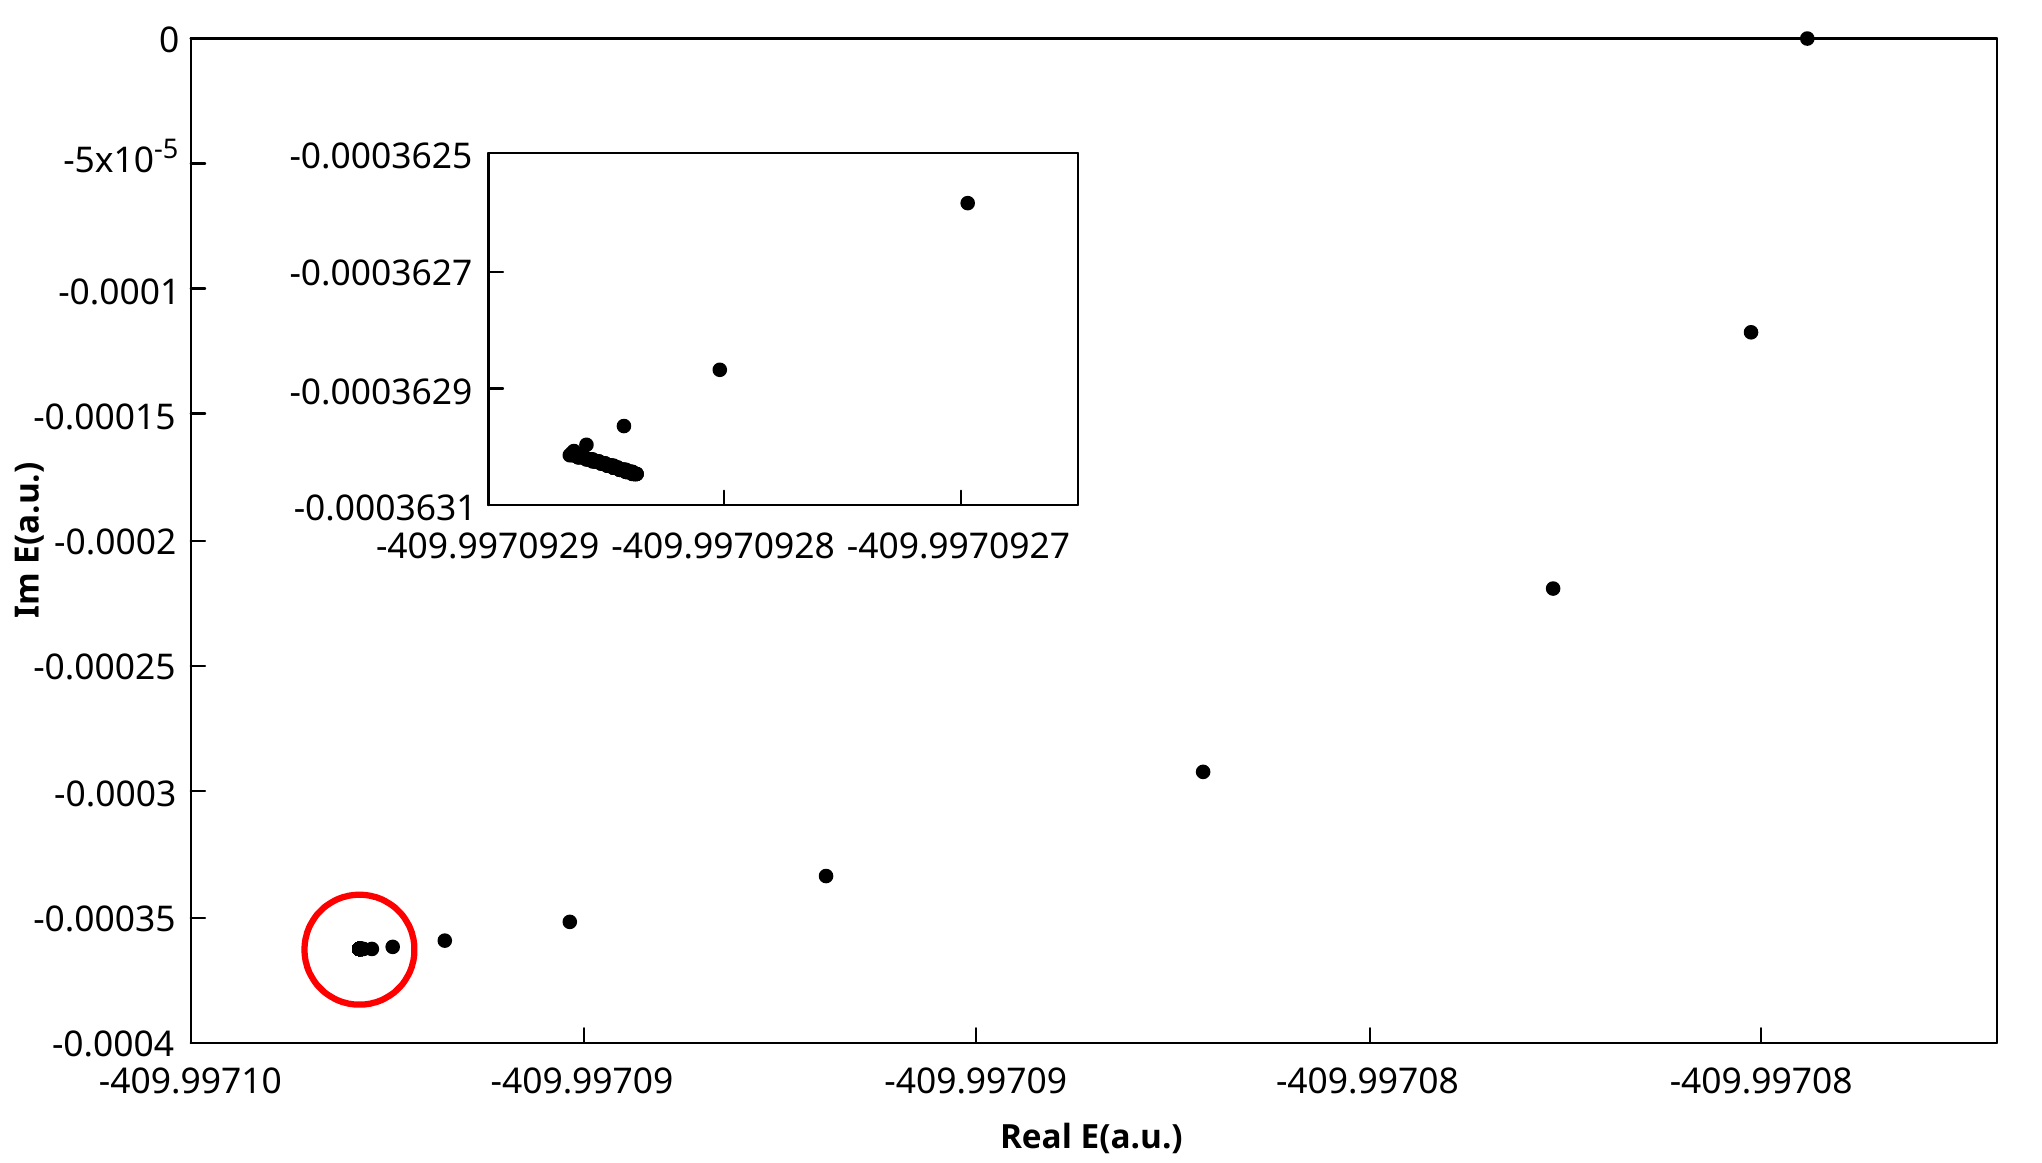}
  \caption{$\theta$-trajectory of resonance with two nodes. The circled potion is zoomed in for clarity.}
  \label{SIfig_14}
\end{figure}

\begin{figure}[H]
\centering
  \includegraphics[width=\linewidth]{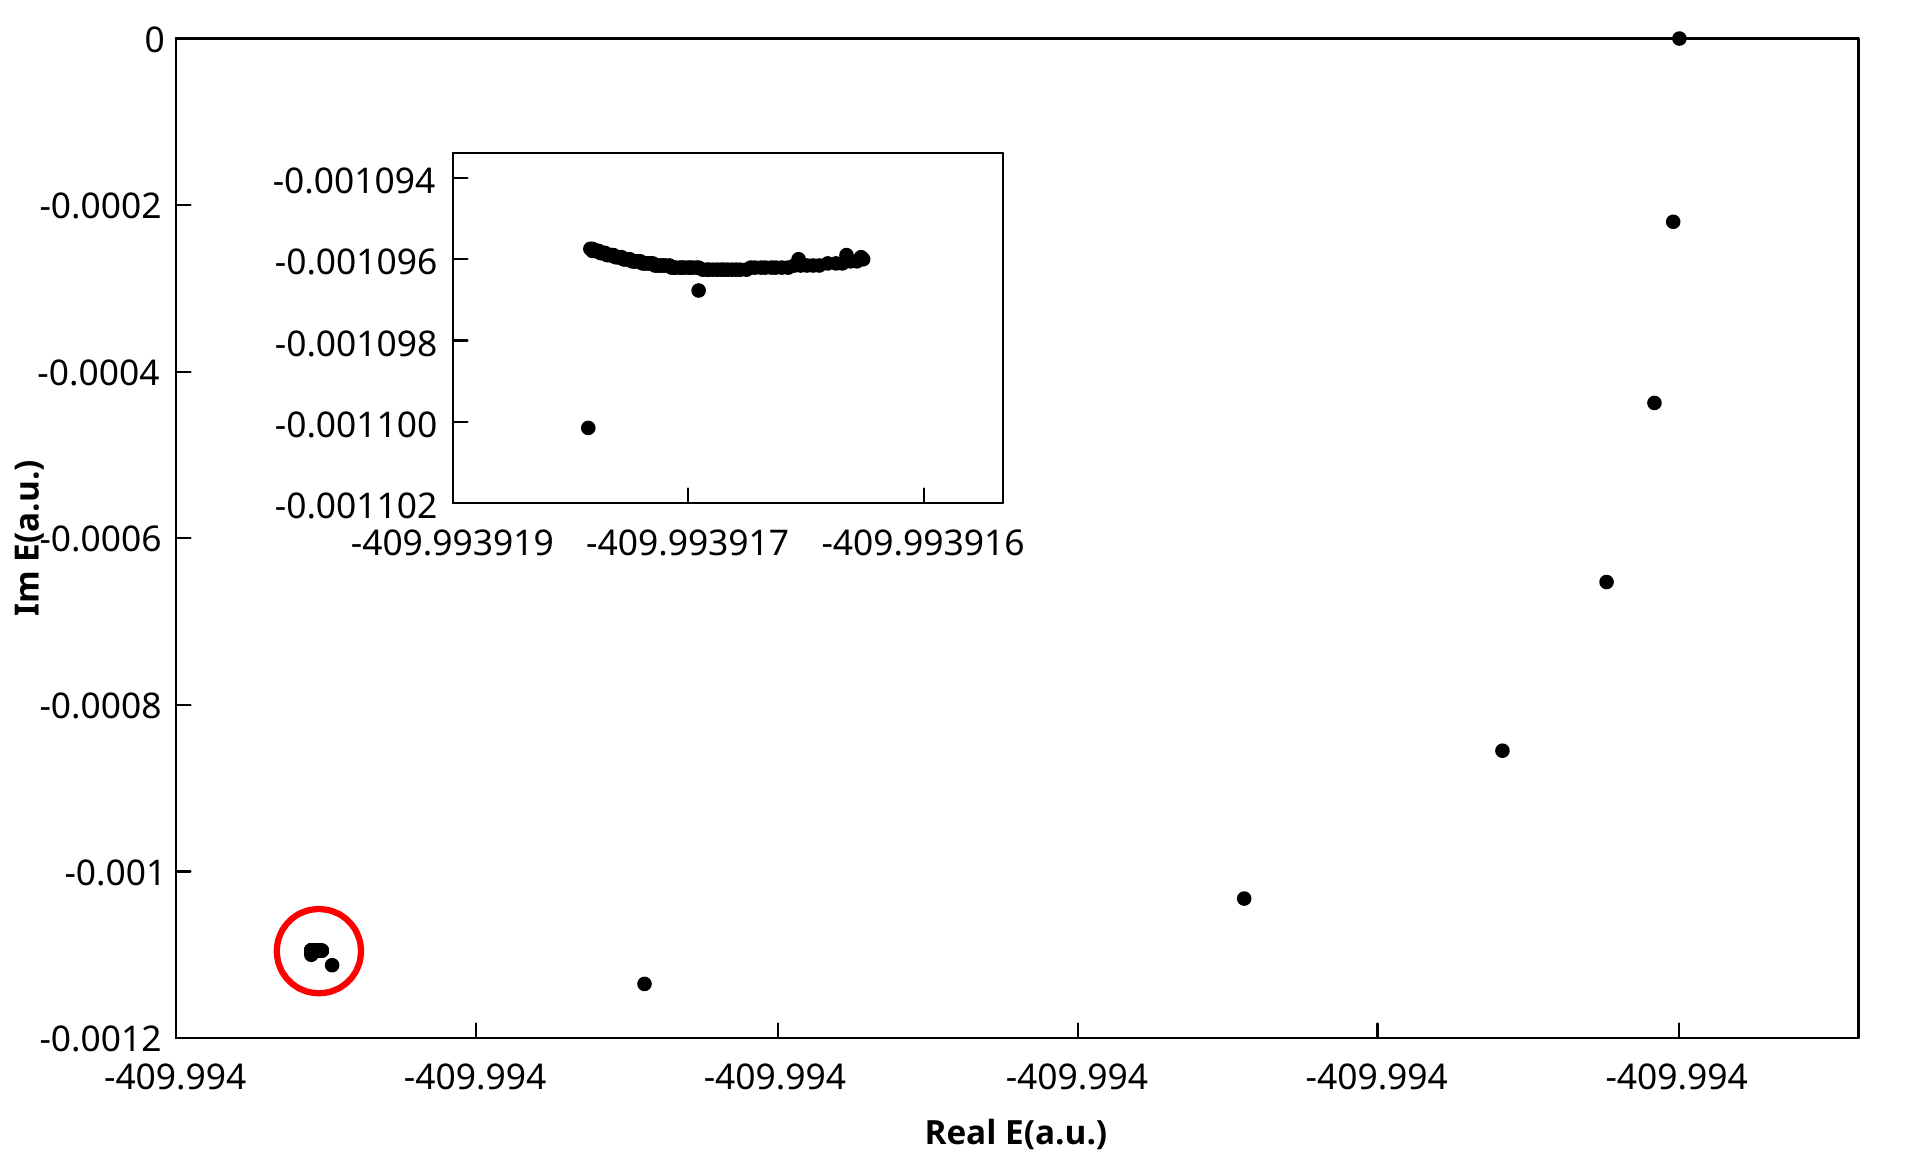}
  \caption{$\theta$-trajectory of resonance with three nodes. The circled potion is zoomed in for clarity.}
  \label{SIfig_15}
\end{figure}

\newpage
Cartesian coordinates and electronic energies (Hartree) of all reported structures

\textbf{O$_{2}$+NO (-280.208894)}\\
 N                  1.23178700   -0.17107400    0.59385900\\
 O                  2.16526500   -0.30904100   -0.07715300\\
 O                 -1.70595600   -0.37276700   -0.21029200\\
 O                 -1.53773900    0.83107100   -0.21586400\\

 \textbf{TS1 (-280.110119)}\\
 N                  0.39368700   -0.04275000    0.37360500\\
 O                  1.43791000   -0.15395400   -0.18038300\\
 O                 -1.18878900   -0.58752400   -0.07342400\\
 O                 -0.59359800    0.77888400   -0.07309700\\
 \textit{978.59$\iota$}\\

 \textbf{INT (-280.118309)}\\
 N                  0.30410300   -0.05644700    0.35668900\\
 O                  1.36596700   -0.24964700   -0.18298200\\
 O                 -0.95310700   -0.59882900   -0.06642600\\
 O                 -0.67914400    0.89789700   -0.06288800\\

 \textbf{TS2 (-280.104560)}\\
 N                 -0.19324000    0.06639900   -0.30249300\\
 O                 -1.20482700    0.63093100    0.03042200\\
 O                  0.26619200   -1.11552200    0.11673700\\
 O                  1.17394500    0.31829600    0.09025800\\
 \textit{2051.87$\iota$}\\

 \textbf{NO$_{3}$ (-280.216796)}\\
 N                 -0.00609200    0.00338200   -0.00139000\\
 O                 -1.07639000    0.61461900   -0.06190300\\
 O                  0.01003200   -1.23681700    0.05243900\\
 O                  1.07199900    0.61892500    0.01050800\\

 \textbf{NO$_{3}$+NO (-410.151281)}\\
 N                 -1.03426900    0.02915600    0.01045600\\
 O                 -1.94249900   -0.75956800   -0.06445800\\
 O                 -1.04117300    1.23605900    0.03672600\\
 O                  2.40627700   -0.20389000    0.00847500\\
 N                  1.42219400    0.38547400   -0.09680300\\
 O                  0.23796000   -0.63540300    0.09481100\\

 \textbf{TS3 (-410.099876)}\\
 N                  1.03191500   -0.00199000   -0.09479900\\
 O                  1.42688100    1.10638600   -0.16037300\\
 O                  1.41808700   -1.11440500   -0.14347600\\
 O                 -2.18735700   -0.00725300   -0.47105300\\
 N                 -1.01788100    0.00338300   -0.20425800\\
 O                 -0.66989100    0.01405300    1.03657500\\
 \textit{638.72$\iota$}\\

 \textbf{2NO$_{2}$ (-410.168240)}\\
 N                 -0.86712600    0.13988600   -0.10598900\\
 O                 -1.18556200    0.22913000   -1.25551600\\
 O                 -1.45348800    0.18665600    0.93555700\\
 O                  1.46916300   -0.16948300   -0.93927700\\
 N                  0.88324700   -0.12264000    0.10251800\\
 O                  1.20225600   -0.21171900    1.25191400\\
